# Supplementary material for: Data Quality Antipatterns for Software Analytics
Source: arXiv:2408.12560 source file (2024-08-22)
Supplement: Supplementary file 1 [file proxy_setup.tex]

# Developer laptop setup <!-- omit in toc -->

This setup should be done in Huawei premises, since working from home requires [additional configuration](#working-from-home) and makes problem debugging harder.

After you laptop is properly setup, you should have:
- WSL 2 installed
- Proxy configured
- SSL certificates installed
- Docker installed
- Huawei mirrors being used whenever possible
- VSCode installed

**Disclaimer**: The instructions shown in this README are provided without any warranty and do not represent or replace Huawei's official instructions. Always double-check things with your supervisor and make sure that you adhere to the company's policies, rules, and guidelines. Happy coding!

# Table of contents <!-- omit in toc -->

- [Install WSL2](#install-wsl2)
- [Setup Ubuntu mirror](#setup-ubuntu-mirror)
- [Setup proxy](#setup-proxy)
- [Install SSL Certificates](#install-ssl-certificates)
  - [Producing the certificates](#producing-the-certificates)
  - [Installing the certificates](#installing-the-certificates)
  - [Making certificates available to other programs (special cases)](#making-certificates-available-to-other-programs-special-cases)
- [Install w3m to test connectivity and SSL](#install-w3m-to-test-connectivity-and-ssl)
- [Install Container Management Technology](#install-container-management-technology)
  - [Option1: Docker](#option1-docker)
  - [Option2: Podman and Podman Compose](#option2-podman-and-podman-compose)
- [Install VSCode](#install-vscode)
- [Install poetry and configure it to create .venv in project](#install-poetry-and-configure-it-to-create-venv-in-project)
- [Working from home](#working-from-home)

## Install WSL2

- Turn on WSL in the windows features:
$ Enable-WindowsOptionalFeature -Online -FeatureName Microsoft-Windows-Subsystem-Linux 

- Install WSL2 and a Ubuntu distribution with the following commands and restart your laptop. (https://learn.microsoft.com/en-us/windows/wsl/wsl-config)

```bash
# install wsl
wsl --install

# check the wsl version
wsl -v

# install lastest Ubuntu LTS as default disto
wsl --install -d ubuntu
```

[Optional] Install Windows Terminal and set it as the default terminal application. (https://learn.microsoft.com/en-us/windows/terminal/install)

**Note**: The instructions shown in this README.md apply for *developer laptop* only. If you are setting up WSL2 on a secure PC, then you likely formal permission from your supervisor. Check the following two URLs:
- http://3ms.huawei.com/hi/group/3764331/wiki_7183031.html
- https://spa.iright-t.huawei.com/#/wf/generalFilingApply?subCategoryCode=1316

## Setup Ubuntu mirror

Check instructions on `http://mirrors.tools.huawei.com`

Then:

```bash
sudo apt-get update
sudo apt-get upgrade
```

## Setup proxy

- A bash file with the following contents:

```bash
#!/bin/bash

# Reading values
PROXY_USER="g00639664"
read -s -p "Enter proxy password: " PROXY_PWD
echo

# Let's define our proxies
export http_proxy="http://$PROXY_USER:$PROXY_PWD@proxyca.huawei.com:8080"
export https_proxy="$http_proxy"
export ftp_proxy="$http_proxy"
export no_proxy=127.0.0.1,localhost,huawei.com,10.193.182.78

# For whatever reason, curl (and some other tools) search for uppercase  
# versions of these variables. So we'd better have them too:
export HTTP_PROXY="$http_proxy"
export HTTPS_PROXY="$https_proxy"
export FTP_PROXY="$ftp_proxy"
export NO_PROXY="$no_proxy"
```

The basic idea is: all traffic that is external to Huawei ("outside world") should go through the proxy. Analogously, internal Huawei websites and servers should be accessed directly (without the proxy).

**Note 1:** The IP `10.193.182.78` in `$no_proxy` is only relevant to the `Software 4.0` research project. That IP is the address of the Kingston1 server (a.k.a., testing server). If your research project accesses servers inside the Huawei network, make sure to add them to the `$no_proxy` variable.

**Note 2:** If you have special characters in your password, they need to escaped. Check [here](https://johndecember.com/html/spec/esccodes.html)

- Load this file using `source [the-script.sh]`. You may also add this line to your `.bashrc` file to ensure that these variables are always loaded in every bash session.

- Once proxy is setup, almost every Linux tool should work fine. Some specific tools however do require proper flags or configuration to work properly. For instance, if you are running `curl`, add the `-L` flag (to allow redirections).

## Install SSL Certificates

### Producing the certificates

Three certificates are needed in total: two for internal Huawei domains and one for external domains. To obtain these three certificates, do the following:
- Certificates for internal Huawei domain: From a Huawei Laptop/Desktop, visit a secure Huawei website (e.g., [CodeHub](https://codehub-g.huawei.com/workspace/projects)) using Chrome. Now, click on the `lock` icon right beside the url, then `Connection is secure`, then `Certificate is valid`. A new popup window will open. Click on the `Details` tab. Select `Huawei IT Root CA` and then click `Export`. Now just save the CRT file (no need to change any settings). Now select `HWIT Enterprise CA 1`, click `Export`, and save the CRT file.
- Certificate for external domains: The process is the same. However, now you need to visit an external website (e.g., [GitHub](https://github.com/openssl/openssl/actions)). The certificate that needs to be saved is called `Huawei Web Secure Internet Gateway CA`.

### Installing the certificates

Copy the three crt files to `/usr/local/share/ca-certificates` and run:

```bash
sudo update-ca-certificates
```

Make sure you see `3 added`. If you see that, it means that the SSL certificates have been successfully installed. Most unix applications will be able to automatically detect these certificates now and SSL problems should disappear (e.g., `self-signed certificate in chain` problems).

### Making certificates available to other programs (special cases)

Not every program running on Linux is able to automatically fetch/consume the certificates that we just installed. Two classic examples are JVM (Java virtual machine) and pip (python package installer).

**- Java**: The easiest way to make SSL certificates available to the JVM is to install the `ca-certificates-java` Ubuntu package:

```bash
sudo apt-get install ca-certificates-java
```

After this package is installed, running the `update-ca-certificates` command will also make all certificates available to the JVM (i.e., certs will be imported into the Java cert keystore).

**- Python's pip**: Python's pip: When running `pip` (or `pip3`), the certificates need to be provided via a `--cert` parameter (see [here](https://stackoverflow.com/a/26062583)). For instance, to install a package from an external domain (e.g., GitHub), the `Huawei Web Secure Internet Gateway CA` needs to be provided. On Ubuntu, all installed certificates can be found under `/etc/ssl/certs`. Example:

```bash
sudo pip3 --cert /etc/ssl/certs/huawei-web-secure-internet-gateway-ca.pem install https://github.com/containers/podman-compose/archive/devel.tar.gz
```

Certificates can also be made available to pip using environment variables. See [here](https://pip.pypa.io/en/stable/topics/https-certificates/#using-a-specific-certificate-store).

## Install w3m to test connectivity and SSL

To assist us in testing the proxy and SSL certificates, let's install `w3m` (a shell web browser):

```bash
sudo apt-get install w3m
```

To test whether Proxy and SSL certificates are working as desired, just try to visit the two following websites. You should be able to view the two websites without any error messages:

```bash
w3m https://codehub-g.huawei.com # internal website
w3m https://www.github.com # external website
```

## Install Container Management Technology

### Option1: Docker

- Follow online instructions here: https://docs.docker.com/engine/install/ubuntu/#install-using-the-repository

- Next, add the following contents to `C:\Windows\System32\drivers\etc\hosts` (open the file as Administrator):

```bash
# Added by Docker Desktop
10.213.123.121 host.docker.internal
10.213.123.121 gateway.docker.internal
# To allow the same kube context to work on the host and the container:
127.0.0.1 kubernetes.docker.internal
```

- Reboot the machine
- Open WSL2
- Do `cat /etc/hosts` and ensure that the changes we've just done to Windows's `host` file are reflected here

- Test docker with the following two commands: 

```bash
sudo docker pull httpd #To check if docker is able to download/pull images
sudo docker run hello-world #To test if docker can download/pull an image AND run a container
```

**Note:** If the test above fails, reach out to Gustavo (g00639664).

### Option2: Podman and Podman Compose

Podman is an alternative to docker. It's key feature is the ability to run 'rootless containers'. Podman offers the exact same commands as docker, since both implement the OCI (Open Container Initiative). It's popularity has increased substantially over the year. However, docker remains the de-facto choice for container management and has a much larger community around it.

- Podman is available from `Ubuntu 23.04` onwards. If you followed the WSL setup instructions, your Ubuntu version will be the latest LTS release. As of today (October 2023), the latest LTS release is `22.04`. Hence, the easieast way to install `podman` right now is to perform an in-place upgrade from `Ubuntu 22.04` to `23.04` (once `24.04 LTS` is out, this problem won't exist anymore). Instructions for in-place upgrade can be found [here](https://askubuntu.com/questions/1459438/how-to-upgrade-ubuntu-22-04-to-23-04).

- Once Ubuntu 23.04 or higher is installed, you can install podman directly from `apt` using `sudo apt-get install podman`.

- To allow podman to pull images without authentication, perform the following commands (more info [here](https://podman.io/docs/installation#add-configuration)):

```bash
sudo mkdir -p /etc/containers
sudo curl -L -o /etc/containers/registries.conf https://src.fedoraproject.org/rpms/containers-common/raw/main/f/registries.conf
sudo curl -L -o /etc/containers/policy.json https://src.fedoraproject.org/rpms/containers-common/raw/main/f/default-policy.json
```

- Test podman with the following two commands (if prompted to pick a registry, pick `docker.io`): 

```bash
podman pull httpd #To check if podman is able to download/pull images
podman run hello-world #To test if podman can download/pull an image AND run a container
```

- Install `podman-compose` by following the instructions from the [official repo](https://github.com/containers/podman-compose). `podman-compose` is 99% compatible with `docker-compose` (same API, same commands).

## Install VSCode

Follow instructions from the official website.

## Install poetry and configure it to create .venv in project

This ensures that VSCode can easily find your Python interpreter

- Install poetry using instructions from [official website](https://python-poetry.org/docs/#installation).
- Configure poetry to create .venv inside project (`virtualenvs.in-project`). See here `https://python-poetry.org/docs/configuration/`

## Working from home

Install wsl-vpnkit: `https://github.com/sakai135/wsl-vpnkit`
