# Supplementary material for: Data Quality Antipatterns for Software Analytics
Source: arXiv:2408.12560 source file (2024-08-22)
Supplement: Supplementary file 2 [file Data_quality_bram_feedback2-FIXED-COMMENTS-REMOVED.pdf]

# Data Quality Antipatterns for Software Analytics

## A Case Study of Software Defect Prediction

Aaditya Bhatia · Dayi Lin ·  
Gopi Krishnan Rajbahadur ·  
Zhen Ming (Jack) Jiang

Received: date / Accepted: date

**Abstract** *Aadi: [check everywhere and add Feature-row imbalance as another antipattern.]*

High-quality data is pivotal for obtaining reliable insights from Software Analytics Machine Learning (ML) models. However, data quality is often compromised by various issues, “data quality antipatterns”, including imbalanced classes, correlation & redundancy, and mislabels. While prior research has identified that these antipatterns can significantly affect the performance and interpretation of ML models, such research have examined these antipatterns in isolation, which may not provide a comprehensive understanding of their overall impact.

In this study, we delve deeper into these antipatterns by examining the case of Software Defect Prediction (SDP), a process that uses the characteristics of old software to predict future code bugness. We aim to provide a holistic view of data quality antipatterns by investigating: a) their prevalence, b) the impact of the order in which they are cleaned, c) their impact on model performance in a setting where the remaining antipatterns have been cleaned out, and d) their influence on model interpretation.

---

Aaditya Bhatia  
Queen’s University, Kingston, ON, Canada  
E-mail: aaditya.bhatia@queensu.ca

Dayi Lin · Gopi Krishnan Rajbahadur  
Centre for Software Excellence, Huawei Canada, Kingston, ON, Canada  
E-mail: {dayi.lin, gopi.krishnan.rajbahadur1}@huawei.com

Zhen Ming (Jack) Jiang  
York University, Toronto, ON, Canada  
E-mail: zmjiang@cse.yorku.ca

Aaditya Bhatia is the corresponding author

Our quantitative analysis reveals that nine antipatterns are prevalent in our studied SDP dataset, with label-based antipatterns co-occurring more frequently. Interestingly, we find that the order of cleaning these antipatterns does not significantly affect the performance of SDP ML models, suggesting that practitioners need not prioritize the sequence of cleaning tasks. Furthermore, while some antipatterns exhibit a statistically significant effect on model performance, most introduce only negligible to small effect sizes. Lastly, our study indicates that models built from data containing different antipatterns present moderately coherent interpretations.

These findings provide empirical guidelines for software analytics practitioners to make informed data-cleaning decisions for their ML tasks, thereby enhancing the reliability of their software analytics.

**Keywords** Data Quality · Machine Learning

## 1 Introduction

Machine Learning (ML) has been widely adopted in various domains of software analytics, including software defect prediction, technical debt identification, and effort estimation [?, ?, ?]. These applications leverage ML to make key decisions, such as predicting future bugs, identifying problematic code, or estimating the required effort for software projects. The reliability of these decisions heavily depends on the quality of the data used to train the ML models [1].

Among these applications, Software Defect Prediction (SDP) is particularly significant due to its widespread use and the criticality of its role in maintaining software quality. SDP has been the focus of numerous studies, and the datasets used in these studies have been reused extensively in the software analytics research community [?, ?]. Therefore, understanding the impact of data quality antipatterns in the context of SDP can provide valuable insights that can be generalized to other areas of software analytics.

While a data quality issue is a recognized problem that has compromise the quality of data, “data quality antipatterns” are potential issues that could become problematic under certain circumstances. These include imbalanced classes, correlation & redundancy, and mislabels. Literature [2, 3, 4, 5, 6, 7, 8, 9, 10, 11, 12, 13] has identified that such antipatterns can significantly affect the performance and interpretation of software analytics ML models. *Bram: [table with name, def citation to how many ..?.. number of aps] Aadi: [we dedicate an entire section to this, where we procure our taxonomy. Should we present that here? –or as a “result” of our taxonomy procurement process?]* Prior studies have examined these antipatterns, but often in isolation, which may not provide a comprehensive understanding of their overall impact [6, 14, 2]. Furthermore, many antipatterns [15, 16] have not been studied in the context of software analytics, despite the widespread use of ML in this field.

Moreover, while it is common knowledge that some antipatterns like tailed distributions [17] or implausible values [2] could exist and impact software an-

*what % ? on cleaned data ?*

alytics, there is no taxonomy or categorization of these antipatterns. This lack of structured understanding of antipatterns further complicates the process of addressing these issues.

Hence, in this study, we address these gaps by developing a taxonomy based on the literature on data quality of seven ML-specific *Bram: [ML-specific or SDP specific?]* *Aadi: [we check the impact of ML-specific the antipatterns on the SDP data. However, the taxonomy is based on ML-specific antipatterns.]* data quality antipatterns, i.e., *Schema Violations*, *Data Miscoding*, *Inconsistent Representation*, *Data Distribution Antipatterns*, *Packaging Errors*, *Label Antipatterns*, and *Correlation & Redundancy*, that contain 12 antipattern subtypes. This taxonomy provides a structured understanding of the potential issues that could affect data quality not only in software analytics, but other fields as well.

We then use software defect prediction (SDP) as a case study to understand the impact of these antipatterns on the performance and interpretation of ML models. This allows us to investigate these antipatterns in a practical, real-world context, and understand their implications on software analytics. Our selected dataset is widely used in other research [18, 19, 20, 21, 22, 23, 24, 25].

Before operationalizing the building of ML models in the context of these data quality antipatterns, we need to address several practical real-world decisions that are not directly answered by prior literature. First, determining the order of cleaning could potentially affect the performance of the models, and understanding the optimal sequence could lead to more efficient and effective cleaning processes. Second, in a setting where other antipatterns are cleaned out, what is the impact of antipatterns on model performance? *Bram: [is this because of ... effects or overlap between integrated data points?]* *Aadi: [we wish to check overlapping effects of the antipatterns.]* Such an understanding is crucial to assess the severity of each antipattern and prioritize our cleaning efforts accordingly. This understanding is exacerbated to assess whether it is worth sacrificing data for cleaning when available data is sparse and the impact of these issues is not significant, i.e., should all antipatterns be cleaned? In some cases, retaining more data, even with some quality issues, might be more beneficial than losing data due to rigorous cleaning.

Finally, interpretation of ML models is a crucial aspect of software analytics, especially when it comes to making informed decisions based on the ML model's predictions. For instance, in software defect prediction, understanding which features contribute most to a prediction can help developers focus their debugging efforts more effectively. Similarly, in effort estimation, interpreting the model can reveal which aspects of a project are likely to require the most resources, enabling better project planning and resource allocation. Despite the importance of interpretation, no research to our knowledge has investigated how data quality antipatterns might affect the interpretation of ML models in software analytics. This gap in the literature presents an opportunity for further exploration and understanding, which we address in this study.

→ i.e., different features considered important?

Overall, we study the following research questions (RQs) in our case study:

- **RQ1: What is the prevalence of data quality antipatterns in software defect prediction data?**

*Results:* SDP data contains *schema violations, correlated and redundant features, distribution antipatterns (tailed and not normal distributions), mislabeling, and duplicated data* antipatterns. We found no instances of *data miscoding, missing values* or the *data drift* antipattern. On the row level, 94% the rows which have more than one antipattern include *mislabels* and *class overlap*. On the column level, 90% of the columns having two antipatterns include *correlated & redundant features* and *tailed features*.

- **RQ2: Does the order of cleaning data quality antipatterns impact the model performance?**

*Results:* Order of cleaning antipatterns has no impact on the performance of the defect prediction models. An antipattern cleaning order pair (say *Mislabel correction (Mi) → Class overlap correction (Ov)*) would have better performance than its inverse order (*Ov → Mi*) in only 50% of the cases which is only random.

- **RQ3: How do data quality anti-patterns impact model performance?**

*Results:* Although five antipatterns (*Tailed, Mislabel, Class Overlap, Class Imbalance, Correlation & Redundancy*) have a statistically significant effect on performance metrics, most antipatterns only introduce a negligible to small effect on the model performance. Among the antipatterns, only the *Tailed* and *Class Overlap* result in a medium or large effect on some of the performance metrics.

- **RQ4: Do models built from different antipatterns give consistent interpretation results?**

Models built from data containing different antipatterns have a moderate interpretation consistency.

*Correlation or causation?*

The remainder of the paper is organized as follows. Section 2 explains the prestudy which summarizes the related work into a taxonomy of data quality antipatterns. Section 3 provides an overview of the case study setup along with a description of the case study parameters and various statistical tests used in this study. Section 4 discusses the motivation, approach, and results for each of our research questions. Section 6 presents the relevant literature in data quality, while Section 5 discusses threats to the validity of our study. Section 7 provides the implications of our findings for researchers and practitioners, Section 8 provides a discussion on our results, and finally, Section 9 concludes the paper.

The findings from this study have implications for practitioners in software analytics. They provide empirical guidelines for making informed data-cleaning decisions for their ML tasks, thereby enhancing the reliability of their software analytics.

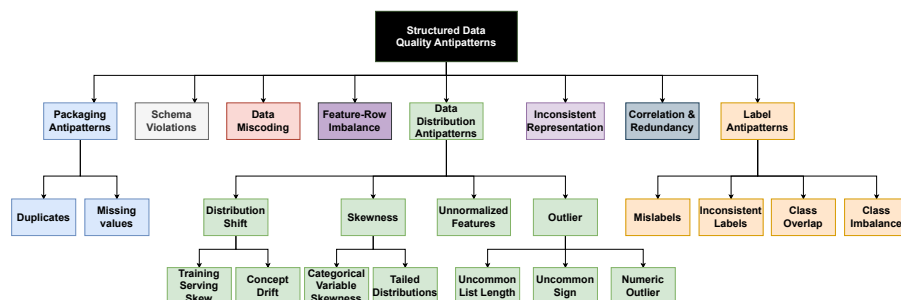

Fig. 1: A taxonomy of data quality antipatterns in structured data. *Bram:* [which of them are new to SDP?] *Aadi:* [We explain this in the results of RQ1.]

## 2 Taxonomy of AI-specific Data Quality Antipatterns

Although previous research has demonstrated the prevalence and impact of various data quality antipatterns, there is currently no comprehensive taxonomy of antipatterns in the literature. In this section, we perform a literature review and summarize data quality into a set of eight broad types, i.e., *Schema Violations*, *Data Miscoding*, *Inconsistent Representation*, *Data Distribution Antipatterns*, *Packaging Antipatterns*, *Label Antipatterns*, *Feature-Row Imbalance*, and *Correlation & Redundancy* of antipatterns, which consist of 12 sub-types.

**Approach.** Our literature review process is as follows. We searched Google Scholar<sup>1</sup> for the terms “data quality”, “data issues machine learning”, “data issues artificial intelligence”, and “data quality artificial intelligence” to obtain an initial list candidate publications relevant to our study. This search was performed exhaustively. *Bram:* [how many results?] *Aadi:* [Unfortunately, I dont have that data, sorry.] *Bram:* [if not discarded, then how many?] *Aadi:* [sorry, this work was lost during laptop transfer.] e., searching for publications until we stop getting any more relevant results by the first and second authors. Along with academic publications, we also referred to industrial tools that fix data quality issues. Our relevancy criterion includes checking whether a candidate publication or industrial tool explains the prevalence, detection, or mitigation of a data quality antipattern. *Bram:* [if not discarded, then how many?] *Aadi:* [sorry, this work was lost during laptop transfer.] As the first step, this paper focuses on structured data quality antipatterns, in the context of ML. Antipatterns for other data types (e.g., images) should be examined in future work. Next, against each candidate publication, we used a lightweight snowballing approach to include relevant publications from the reference list. *Bram:* [how many extra hits?] *Aadi:* [sorry I dont have that info now.] The first, and the second authors discussed to logically group the found antipatterns into a taxonomy using a card-sorting like method.

<sup>1</sup> scholar.google.com

*Explain (in particular disagreement between both notes)*

*reviewers will ask this*  
*any way to approximate these numbers?*

*how searched?*  
*how so?*

**Results.** We identified a total of eight high-level types of antipatterns, which consist of a total of 12 sub-types. Figure 1 presents a taxonomy of the eight high-level data quality antipattern types along with their 12 sub-types.

– **Schema Violations.** *Bram: [vague example + citation to main sources?]*

Schema identifies a blueprint for the organization of the data. This blueprint is based on a set of rules. Violations of the rules that explain the logic of the objects/associations/entities described by the data are schema violations. For relational databases, integrity constraints are enforced to ensure the correctness of data within a defined schema. However, violations can occur if such rules are not enforced or are undefined. Schema violations are quality antipatterns as data that violate schema are likely to be inaccurate and therefore introduce noise to the pattern that ML models are trying to learn. Schema rules have been proposed and used for data cleaning in the literature. For instance, in the context of defect prediction, *number\_lines* (total lines of in a source code file)  $\geq$  *number\_blank\_lines* (lines which have no code or comments, and are left blank) is a schema rule [2].

**Data Miscoding.** Data miscoding refers to an incorrect data type used while training the ML model. While performing data-wrangling tasks, this antipattern can be dynamically introduced. For instance, an *enum* can be incorrectly read as a *real number* in the memory. We consider miscoding as an antipattern as models trained from such incorrect data types may learn improper information from the miscoded features.

Hynes et al. [17] explained other manifestations of data miscoding as *numbers as strings*, *tokenizable strings*, *circular domain as linear*, *date/time as a string*, *zip code as a number*, and *integer as float*. Gitzel et al. [15] identified manifestations of miscoding in *time-series* datasets. Removing this antipattern is a vital common practice, and to combat this antipattern, researchers and practitioners explicitly typecast during the data preprocessing steps performed before building ML models. For instance, Sharma et al. [3] mentioned “all the incorrect data types of the features changed to their required datatype” while evaluating ML-based feature selection approaches for breast cancer detection.

- **Inconsistent Representation.** Two or more ways of representing the same concept within the data. For instance, in a dataset with a country code feature, countries like Canada could be represented by the string “CAN” in some entries while “CANADA” or lower case string “canada” or a camel case “Canada” in others leads to inconsistent representations. This antipattern can also manifest as an inconsistency with the alphabet case for a string feature. In time series data, this antipattern could manifest as inconsistent units (e.g., cm and inches) for the same feature [15].
- **Data Distribution Antipatterns.** Several characteristics of distributions have been considered as antipatterns by prior research [17, 4]. We observed seven sub-types of distribution errors from the literature.

*in CSV files*

*building a dataset, loading, writing*

- **Unnormalized Features.**<sup>2</sup> Distribution of a feature that is widely different from the distribution of other features.
- **Outliers.** Under the sub-category of outliers, we have further sub-categories based on the type of outlier, i.e., size, numerical outlier, or sign. We provide a definition for each below:
  - **Tailed Features.** Extreme values that significantly affect mean are tailed [17]
  - **Uncommon list length.** For features composed of lists, some instances have a different length than the common or correct length [17].
  - **Uncommon sign.** For numeric features, some values having different sign (+/-) from the rest of data [17]. Particularly, the sign of a feature itself is an outlier.
- **Training serving distribution skew.** A difference between the distribution of data used during model training phase and deployment (a.k.a. serving) phase. *Bram: [issue of data, ml scripts or of data points] Aadi: [issue of data being differently distributed]*. When these data distributions are significantly different (i.e., there is a heavy “skew”), the model can perform poorly on the new data [4]. Training-serving skew is considered an antipattern because if the data used to train the model does not accurately represent the data that the model will encounter in production, it may result in issues such as overfitting, bias, or poor performance.
- **Data drift.** Drift is a distribution change between different snapshots of data, which can be problematic if models trained on those differently distributed datasets have performance changes. Data drift could be prevalent in both independent and dependent features [26, 5]. *Covariate drift* occurs when there is a shift in the independent variables over time. For instance, a cats/dogs classifier trained on images of golden retrievers has a change in deployment, where a newer breed of dog, say bulldog, is introduced. *Bram: [this is antipattern across data points?] Aadi: [yes, this is across data points compared during different time periods.]* *Class drift a.k.a. prior probability drift:* shift in the target variable. For the cats/dogs classifier, class drift could manifest as the addition of an entirely new class, say rabbit images.
- **Constant Features.** Features that have no variance or have the same value for all rows. These features do not add any value to the ML model and hence, Constant features are an antipattern.
- **Packaging Antipatterns.** As mentioned by Hynes et al. [17], “Packaging errors identify problems with the organization of the data”. These issues have the potential to seep into the dataset while packaging the data for building ML models, perhaps during the data preprocessing step of the ML pipeline [27]. Packaging errors manifest as *Empty* or *Duplicated* values.

---

<sup>2</sup> We use the definition of Unnormalized features from [17]. This is not the same as Not Normal (i.e., Not Gaussian) distributions.



- **Empty Values.** Missing or null values must be dealt with before using the data for ML tasks, since ignoring or omitting missing values may result in biased or misinformed analysis [28].
- **Duplicates.** Repeated entries for one or more features [29, 17, 2]
- **Label Antipatterns.** Antipatterns with the dependent variables associated data for supervised learning tasks.
  - **Inconsistent Labeling.** Values correspond to the same label but have different and inconsistent labeling strategies. In the case of labels assigned via crowd-sourcing (i.e., organizations employ large teams to annotate ML datasets), inconsistencies in the labeling strategy employed by different teams can cause performance issues for ML models [30]. Similar issues can occur with non-human labeled datasets labeled with inconsistent strategies [29].
  - **Mislabels.** Response variable labeled via an incorrect labeling strategy. As opposed to *inconsistent labeling*, mislabels antipattern includes incorrectly assigned labels. In the case of SDP, Da Costa et al. [31] suggested improving the approach to label bug-introducing commits. Indeed, their labeling strategies lead to performance improvements for SDP models, as identified by Yatish et al. [32].
  - **Class Overlap.** The instances that have similarities in feature values although they belong to different classes and such a complication is a substantial obstacle in their classification [8]. These instances have more than one class sharing a common region in the data space. The adverse impact of Class overlap often goes hand in hand with Class imbalance [6, 7, 8, 9].
  - **Class Imbalance.** This antipattern occurs when the majority of instances are labeled with one class, whereas very few instances are labeled with the other class(es) [33]. Class imbalance significantly impacts the performance of ML classifiers [10, 11, 12]
- **Correlation & Redundancy.** We identify *correlation* & *redundancy* as one antipattern group since their presence while training ML models renders the model's interpretation inconsistent, as identified by Jiarapakdee et al. [34]. Following Juarpakdee's seminal work in 2019, future defect prediction research (e.g., [35, 36, 9]) has removed correlated and redundant features before performing ML tasks. An explanation of *correlation* & *redundancy* is provided below:
  - **Correlation.** A relation between two or more variables. When variables are too closely related (i.e., correlated), it can lead to multi-collinearity. Its crucial to remove correlated variables before ML model training [13].
  - **Redundancy.** One or more independent variables being represented by other independent variables. Redundant variables interfere with each other, distorting the modeling relationship between the independent and the dependent variables. Hence, such variables need to be removed before training the ML model [14].
- **Feature-row imbalance**



For training ML models, the data size should be in moderation, where too many features w.r.t. the number of rows or vice-a-versa cause model performance issues. We explain both these cases below:

- **Over-dimensionality** antipattern cause issues that are commonly attributed to as “Curse of Dimensionality”. The number of dimensions (features) are much large as compared to the number of observations (samples/rows). Prior research [37,38,39] has attributed issues such as poor classification accuracy, overfitting, decreased model interpretability, and increased computational time/resources to the curse of dimensionality.
- **Under-dimensionality** is a feature-row imbalance where there are much more rows than features (dimensions). Such situations cause ML model underfitting, leading to high model bias, and potential data redundancy (i.e., with too many rows, patterns usually start to be repetitive [40,41]).

### 3 Case Study Setup

In this section, we describe the case study setup that is used to answer the research questions.

#### 3.1 Studied Dataset

*Bram: [to justify non-deep learning, refer to paper of Jack, Zheng, Deep just in time defect prediction : how far are we? 2021 ACM sigsoft] Bram: [how big is the data? how many data points?] Aadi: [the defect prediction done by Kla (yatish et al.) does not align with JIT defect pred. Yatish focused on post-release. – or am I missing your point??]* In this study, we use the software defect prediction dataset from Yatish et al. [32]. Software defect prediction is the process of identifying and forecasting potential errors in software applications before they occur. We use software metrics as explanatory and response variables, helping to identify patterns and correlations that can predict future software bugs, improving the quality of future releases. These metrics are both code related (i.e., metrics that define the relationship between code properties and software quality) and process related (i.e., metrics that define relationship between development activities and software quality) [32]. Table 1 presents 65 metrics that are adapted from Yatish et al. and used in this study. The study by Yatish et al., which delved into the characteristics of the response label in SDP, can be interpreted in our study context as an effort towards “mislabel correction”. The dataset comprises of nine projects from popular libraries and their 30 project versions as shown in Table 2.

*(agreed)*

→ mention that file-level prediction  
+  
need to justify why no deep learning model was trained by citing papers like...

Table 1: Metrics from our studied SDP dataset obtained from Yatish et al. [32]  
*Bram: [do we need definitions? Aadi: [Yatish's paper itself doesnt provide defi for each metric, they just said they obtained metrics from Scitools, and provide defi for the metric type. Moreover, Scinet metric definitions are also dumb (eg, MaxNesting is the maximum of nestings in all functions), then they provide a code example. Also Yatish's dataset is fairly common for SDP. The papers using this dataset dont provide metric defi too.]]*

| Metric Type         | Metric Names                                                                                                                                                                                                                                                                                                                                                                                                                                                                                                                                                                                                                                                                                                                                                                                            |
|---------------------|---------------------------------------------------------------------------------------------------------------------------------------------------------------------------------------------------------------------------------------------------------------------------------------------------------------------------------------------------------------------------------------------------------------------------------------------------------------------------------------------------------------------------------------------------------------------------------------------------------------------------------------------------------------------------------------------------------------------------------------------------------------------------------------------------------|
| Granularity Metrics | AvgCyclomatic, AvgCyclomaticModified, AvgCyclomaticStrict, AvgEssential, AvgLineBlank, CountDeclClassMethod, AvgLineCode, Avg-LineComment, AvgLine, CountDeclClassVariable, CountStmt, CountDeclFunction, CountDeclInstanceMethod, CountDeclInstanceVariable, CountDeclMethod, CountDeclMethodDefault, CountLine, CountDeclMethodPrivate, CountLineBlank, CountDeclMethodProtected, CountDeclClass, CountDeclMethodPublic, CountLineCode, CountLineCodeDecl, CountLineCodeExe, CountLineComment, CountSemicolon, CountStmtDecl, CountStmtExe, MaxCyclomatic, MaxCyclomaticModified, MaxCyclomatic-Strict, RatioCommentToCode, SumCyclomatic, SumCyclomaticModified, SumCyclomaticStrict, SumEssential, CountClassBase, CountClassDerived, MaxInheritanceTree, PercentLackOfCohesion, CountClassCoupled, |
|                     | CountInput {Min, Mean, Max}, CountOutput {Min, Mean, Max}, CountPath {Min, Mean, Max}, MaxNesting {Min, Mean, Max}                                                                                                                                                                                                                                                                                                                                                                                                                                                                                                                                                                                                                                                                                      |
|                     | COMM, ADDED_LINES, DEL_LINES,                                                                                                                                                                                                                                                                                                                                                                                                                                                                                                                                                                                                                                                                                                                                                                           |
| Process Metrics     | ADEV, DDEV,                                                                                                                                                                                                                                                                                                                                                                                                                                                                                                                                                                                                                                                                                                                                                                                             |
| Ownership Metrics   | MINOR_COMMIT, MINOR_LINE,                                                                                                                                                                                                                                                                                                                                                                                                                                                                                                                                                                                                                                                                                                                                                                               |
|                     | MAJOR_COMMIT, MAJOR_LINE, OWN_COMMIT, OWN_LINE                                                                                                                                                                                                                                                                                                                                                                                                                                                                                                                                                                                                                                                                                                                                                          |

| Project Name | Version# | Median Row# |
|--------------|----------|-------------|
| Activemq     | 5        | 2040        |
| Camel        | 2        | 7517        |
| Derby        | 3        | 2206        |
| Groovy       | 3        | 821         |
| Hbase        | 3        | 1669        |
| Hive         | 3        | 1560        |
| Jruby        | 4        | 1054.5      |
| Lucene       | 4        | 1325.5      |
| Wicket       | 3        | 1763        |

Table 2: The studied project data, version count and the data size.

### 3.2 Antipattern Detection Techniques

In this sub-section, we outline the procedure for checking different data quality antipatterns within our studied SDP dataset. we describe the approach to detect each of these data quality antipatterns below.

Table 3: Schema Violation Rules. Rules marked with an asterisk(\*) are domain-specific.

| Rule | Rule Description                                                                                                                                           | Rule Pseudo-Code                                                                    |
|------|------------------------------------------------------------------------------------------------------------------------------------------------------------|-------------------------------------------------------------------------------------|
| R1*  | All metrics should be greater or equal to zero                                                                                                             | Metric $\geq$ 0                                                                     |
| R2*  | #physical lines should be greater than or equal to the #lines containing comments.                                                                         | CountLine $\geq$ CountLineComment                                                   |
| R3*  | #physical lines should be greater than or equal to the average lines of code.                                                                              | CountLine $\geq$ AvgLine                                                            |
| R4*  | #physical lines should be greater than or equal to the #declarative lines of code.                                                                         | CountLine $\geq$ CountLineCodeDecl                                                  |
| R5*  | #physical lines should be greater than or equal to the #executable lines of code.                                                                          | CountLine $\geq$ CountLineCodeExe                                                   |
| R6*  | #physical lines should be greater than or equal to the sum of declarative and executable lines of code.                                                    | CountLine $\geq$ CountStmt                                                          |
| R7*  | #physical lines should be greater than or equal to the #blank lines of code.                                                                               | CountLine $\geq$ CountLineBlank                                                     |
| R8*  | #physical lines should be greater than or equal to the sum of their components, i.e., sum of blank lines, comment lines, declarative and executable lines. | CountLine $\geq$ (CountLineBlank + CountLineComment + CountLineDecl + CountLineExe) |
| R9*  | #statements should be the sum of declarative statements and executable statements.                                                                         | CountStmt = CountLineCodeDecl + CountLineCodeExe                                    |
| R10* | The ratio of comment to code should be the #comment lines divided by the total #code lines.                                                                | RatioCommentToCode = Comment-LineCode / CountLineCode                               |
| R11* | For all nested functions or methods, average physical lines should be greater than the average lines containing code.                                      | AvgLine $\geq$ AvgLineCode                                                          |
| R12* | For all nested functions or methods, average physical lines should be greater than the average lines containing comments.                                  | AvgLine $\geq$ AvgLineComment                                                       |
| R13* | For all nested functions or methods, average physical lines should be greater than the average lines containing blank lines.                               | AvgLine $\geq$ AvgLineBlank                                                         |
| R14* | For all nested functions or methods, average physical lines should be greater than the sum of average lines containing code, comments, and blank lines.    | AvgLine $\geq$ (AvgLineCode + Avg-LineComment + AvgLineBlank)                       |
| R15  | For all nested functions or methods, the sum of cyclomatic complexity should be greater than the maximum cyclomatic complexity.                            | SumCyclomatic $\geq$ MaxCyclomatic                                                  |
| R16  | For all nested functions or methods, sum of strict cyclomatic complexity should be greater than the maximum strict cyclomatic complexity.                  | SumCyclomaticStrict $\geq$ MaxCyclomaticStrict                                      |
| R17  | For all nested functions or methods, sum of modified cyclomatic complexity should be greater than the maximum modified cyclomatic complexity.              | SumCyclomaticModified $\geq$ MaxCyclomaticModified                                  |
| R18  | For all nested functions or methods, maximum of cyclomatic complexity should be greater than the average of cyclomatic complexity.                         | MaxCyclomatic $\geq$ AvgCyclomatic                                                  |
| R19  | For all nested functions or methods, maximum of strict cyclomatic complexity should be greater than the average of strict cyclomatic complexity.           | MaxCyclomaticStrict $\geq$ AvgCyclomaticStrict                                      |
| R20  | For all nested functions or methods, maximum of modified cyclomatic complexity should be greater than the average of modified cyclomatic complexity.       | MaxCyclomaticModified $\geq$ AvgCyclomaticModified                                  |

only for "nested" !

### 3.2.1 Schema Violations

A schema, refers to a predefined rules and structures that dictate the acceptable values and relationships for data. These rules help identify and rectify implausible or erroneous data points. Since there is no formal definition of software defect prediction schema rules in academia, we first formulate a schema for our studied SDP data, then check for deviancy from the logic defined within these rules. Our approach for finding schema rules is two-phased. Firstly, we referred to prior literature to check the rules and associations between the SDP metrics. For instance, Shepperd et al. [2] defined referential integrity checks (like  $\#LINES \geq \#CODE + \#COMMENT$ ) for NASA dataset. In total, we observed that seven out of the 18 rules *Bram: [affecting all ~~domain~~ groups of metrics?]* *Aadi: [not sure what this comment means?]* defined by Shepperd et al were applicable to our dataset, and reused them. Next, we analyzed the definitions for each metric defined in Table 1 to develop more rules. Finally, we used statistics knowledge of i) sum of a metric is greater or equal to the max value, ii) maximum should be greater or equal to the average value, to generate statistics-based rules.

Table 3 presents a set of 20 identified rules with a unique identifier for every rule. R1-R14 are domain-specific (SDP domain) rules and are marked with \*, whereas, the remaining rules (i.e., R15-20) are based on common statistics. *Bram: [what about between metrics, do we have rules for them?]* *Aadi: [yes, the domain specific rules are based on metric definitions]*

In the table, Rules like R9 (indicating that the “#total statements” should be the sum of “declarative” and “executable” statements) are based on the metric definitions obtained from Scitools<sup>3</sup>. In particular, *declarative* statements include variable assignment (e.g., `x=10;`) and executable statements include method calls (e.g., `System.out.println("Hello, World!");`). On the contrary, rules like R18 is based on the statistical rule of maximum value should be greater than the average value.

### 3.2.2 Distribution Antipatterns

We use Hynes et al.s [17] implementation to identify unnormalized features, and tailed features.

- **Constant Features.** We identify constant features by checking whether the variance of a feature is zero. Such an approach can only be adopted for numerical features. We do not have any categorical features within our studied SDP data and hence, have not adopted any technique to remove any constant categorical feature.
- **Data Drift.** For each project in our studied SDP dataset, we detect drift between its consecutive versions. For instance, to detect data drift for the project *Derby* having versions, *10.2.1.6*, *10.3.1.4*, and *10.5.1.1*, we study

<sup>3</sup> <https://support.scitools.com/support/solutions/articles/70000582223-what-metrics-does-understand-have->

*pairwise*

drift between i) *10.2.1.6 and 10.3.1.4*, ii) *10.3.1.4 and 10.5.1.1*. Our approach employs TFDV's (tensorflow data validation tools) implementation to detect this drift. Notably, we compared the consecutive version-comparison for each project includes five versions of *activemq*, four versions of *camel*, three versions of *derby*, three versions of *groovy*, three versions of *hbase*, three versions of *hive*, four versions of *jruby*, four versions of *lucene*, and three versions of *wicket*.

- **Unnormalized Distributions.** The calculation involves trimmed means (the mean calculated after removing the top and bottom 10% of data points, which may include extreme low or high values) and standard deviations for these features, thereby discounting extreme values at both ends of the spectrum. This approach focuses the analysis on more representative central data points. For each numeric feature, the detector assesses the deviation of its mean and standard deviation from these trimmed statistics using z-score calculations. Features whose mean or standard deviation deviances exceed a certain threshold<sup>4</sup> are considered unnormalized.
- **Tailed Distributions.** This implementation relies on checking whether the deviation of a feature mean is greater than that of its trimmed mean. Hynes et al's implementation detects custom missing/placeholder values (e.g., -999), along with finding obvious statistical outliers.

i.e., all version information!

### 3.2.3 Package Antipatterns

- **Empty Values.** We use the pandas `isnull`<sup>5</sup> function to check for empty values.
- **Duplicates.** In our SDP dataset, a row represents a source code file within a specific project version. If that file has the exact feature values as another file, then such files (rows) are duplicated. We bring the data in the same format as that of explanatory variables, and detect duplicates on a row level using the `duplicated()` function<sup>6</sup> from Pandas package.

### 3.2.4 Label Antipatterns

- **Mislabels.** Yatish et al.'s [32] dataset consist of labels (i.e., whether a file is buggy) from two strategies. At the core of data preparation for SDP is the identification of post-release defects (i.e., modules that are changed to address a defect report after software is released). The traditional approach for identifying post-release defects involves extracting specific keywords and issue IDs from commit logs in the version control system (VCS) using regex [42,43]. This information is then used as the label for ML models to predict the bugginess of new or future code. Yatish et al. improved upon this traditional approach by adopting suggestions from Da Costa et al.'s [31]

<sup>4</sup> We use the default threshold values obtained from [17]

<sup>5</sup> <https://pandas.pydata.org/docs/reference/api/pandas.isnull.html>

<sup>6</sup> <https://pandas.pydata.org/docs/reference/api/pandas.DataFrame.duplicated.html>

to consider affected releases in an issue-tracking system when identifying defect-introducing commits. The realistic (correct) approach involves taking the release information for identifying bug-introducing commits. This stands in comparison to the (mis)labeled “heuristic” approach which relies on traditional methods of generation of bug-introducing commits. We use the “RealBug” and the “HeuBug” feature names from Yatish’s dataset to identify correct and mislabeled tuples respectively.

- **Class Imbalance.** We determine the presence of class imbalance by evaluating the ratio of the minority class with respect to the overall size of the data for each project-version of the SDP dataset.
- **Class Overlap.** We use the Gong et al.’s [9] improved K-Means clustering cleaning approach (IKMCCA) to detect rows with overlapping classes for each project version of the SDP data. This approach solves both class overlap and class imbalance problems by combining the K-Means clustering cleaning approach (KMCCA) [44] and the Neighbourhood cleaning technique (NCL) [6]. IKMCCA removes overlapping instances based on the percentage of defective instances. After performing K-means on the explanatory variables, IKMCCA checks if the percentage of defective instances in the  $i_{th}$  cluster lies below a threshold  $p\%$ , then the cluster’s defective instances are removed, otherwise, the non-defective instances for that cluster are removed.

Our studied dataset contains mislabeled variable (“*RealBug*”) and correctly labeled variable (“*RealBug*”). Since class overlap is depends on the labels, we use the corrected labels in **RQ1**, and use the correct or mislabeled variables depending on the order of cleaning for building models in **RQ2** and **RQ3**.

why does this solve this issue?

### 3.2.5 correlation & redundancy *isn't that result of last RQ?*

Due to their impact on the model interpretation, we consider both correlation & redundancy into one group, and detect them together. Before building ML models, removing correlated and redundant features involves selection of features that are most important to the data scientist. To serve this purpose for our SDP data, we use the R package RNalytica [45] that automatically selects important features for SDP data [46]. This preprocessing step is popularly used in software engineering research [32, 35, 47, 48].

what algorithm?

## 3.3 Feature-Row Imbalance

We check the ration of features (columns) and the samples (rows) for each project version of our studied SDP dataset.

### 3.4 Constructing Defect Models

In this subsection, we discuss the different aspects of constructing ML models for **RQ2** and **RQ3**.

#### 3.4.1 Studied Learners

For **RQ2** and **RQ3**, we construct ML models using four learners, namely, *Neural Network* (NN), *Logistic Regression* (LR), *Random Forest* (RF), and *XG-Boost* (XGB). These learners are chosen as they represent the prominent families of learners [49] *Bram: [for families see that Jack paper about deep learning] Aadi: [they seem to use logistic regression—what change is required here? (sorry for missing your point)]* used in defect prediction. Specifically, we select learners from the Bagging, Boosting, Regression, and Neural Network families respectively. We excluded the learners from families such as Naive Bayes, Nearest Neighbors, Discrimination analysis, Rule-based, and SVM since these learners are known lack of performance in defect prediction [50,51]. Since we already use the random forest classifier which is an aggregation of decision trees, we exclude the decision tree classifier in our study. Additionally, the Partial Least Squares family, which is a dimensionality reduction technique, was not included as it is not directly applicable to classification tasks.

we need to justify choice of non-deep learning

#### 3.4.2 Hyper-parameter tuning

For each of the models built in **RQ2** and **RQ3**, we search for the optimal hyperparameters after performing the respective data cleaning techniques for **RQ2** and **RQ3**. We perform hyperparameter tuning keeping the *#iterations* = 10 (i.e., 10 different sets of hyperparameters were evaluated) using the Random Searching algorithm. The “random search” algorithm is more efficient than its alternative, “grid search” in estimating the optimal hyper-parameters [52]. We kept the cross validation parameter as 3 (i.e., 33% data was used as validation set).

To obtain a range of tuning the hyperparameters of the studied classifiers, we refer to SOTA literature on hyperparameter optimization in SDP, and our range of tuned hyperparameters is provided in Table 4. Specifically, We obtain a list of hyperparameters for each the Logistic regression and the Random Forest learners from Aggarwal et al. [53]. XGB hyperparameters are obtained from Alazba et al. [54], while the Neural Network parameters are used from Bhaweres et al. [55].

why cross-validation?  
↓  
are just for hyperparameter tuning (on validation set?)

#### 3.4.3 Model Validation

We split 80% of the data into training and 20% into testing using stratified sampling to ensure that there are instances of buggy and non-buggy classes in both sets. *Bram: [no crossvalidation?] Aadi: [No. hyperparameter tuning data (validation) was randomly taken out of the training data 10 times from*

we need figure to clarify the train / valid / test data sets used



Table 4: Hyperparameter parameters for all learners used in this study.

| learners            | Hyper parameters                                                                                                                                                     |
|---------------------|----------------------------------------------------------------------------------------------------------------------------------------------------------------------|
| Random Forest       | Criterion: [gini, entropy]<br>N_estimators: randint(50, 150, 250, 500, 750)<br>Min_samples_split: randuniform(0,0.1)                                                 |
| Logistic Regression | Penalty : [l2, none],<br>C : random int (1, 500)                                                                                                                     |
| Neural Network      | Learning_rate: randuniform(0.001, 0.01)<br>Dropout: randuniform(0.1,0.5)<br>Neurons: randint(25,100)<br>Hidden_layers: randint(1,5)<br>Batch_size: [64], Epoch: [15] |
| XGB                 | N_estimators: [100,50,500,1000]<br>Max_depth: [6,3,4,5]                                                                                                              |

*the same training data. Randomness in validation set prevents overfitting. Updated the hyper-parameter tuning subsection to make it more explanatory. ]*  
 This split is done 10 times, with ML models built on each split to obtain the performance metrics. Although bootstrapping is considered a robust validation strategy [35], sampling with replacement leads to duplication of data in the training set. This does not allow us to assess the impact of *Duplication* as a data quality antipattern, restricting our use of bootstrapping as a validation technique.

#### 3.4.4 Performance Estimation

For each of the ML models built in **RQ2** and **RQ3**, we evaluate the performance of the SDP models using the two threshold dependent and four threshold independent metrics given below.

- **AU-ROC** or *Area Under the Receiver Operator Curve* is a threshold-independent metric. While calculating the performance of a classifier, a threshold classifies the outcome as “defective” or “non-defective”. AU-ROC measures the area under the curve at all thresholds of the receiver operator curve which plots the true positive rate (sensitivity) against the false positive rate ( $1 - \text{Specificity}$ ).
- **AU-PRC** is another threshold-independent metric that calculates the *Area Under the Precision-Recall Curve* at different thresholds. AU-PRC is beneficial for cases where the positive class (like the presence of software bugs in our case) is more valuable to determine than the negative class (i.e., not buggy clean code), and is a better estimate for datasets suffering from the class imbalance antipattern [56].
- **Pr** or *Precision* estimates the observations correctly predicted out of all predictions. It’s calculated as  $\text{True Positives} / (\text{True Positives} + \text{False Positives})$ . *Bram: [not reliable when imbalanced, need g-mean] Aadi: [fair, but 1) we don't have that bad class imbalance as per RQ1 2) even with high imbalance, only AUPROC and AUC are reliable. Youdgen J stat metric or*

*g-mean based threshold balancing is also not also reliable (citation: Hancock, John T., Taghi M. Khoshgoftaar, and Justin M. Johnson. "Evaluating classifier performance with highly imbalanced Big Data." Journal of Big Data); that's why we provide the threshold independent metrics. We do explicitly mention that independent ones are not-reliable for model performance, but may be valuable to certain type of practitioners.]*

- **Re** or *Recall* estimates the observations correctly predicted over the total number of correct observations. It's calculated as  $\text{True Positives} / (\text{True Positives} + \text{False Negatives})$ .
- **F1 Score** strikes a balance between Precision and Recall by calculating the harmonic mean between the two. Its calculated as  $2(\text{Pr} * \text{Re}) / (\text{Pr} + \text{Re})$
- **MCC** or *Mathews Correlation Coefficient* (MCC) is considered as a reliable metric [57] as it produces good scores only if the prediction returns good rates for true positives (TP), true negatives (TN), false positives (FP), and false negatives (FN). MCC is calculated as  $(TP * TN - FP * FN) / \sqrt{(TP + FP)(TP + FN)(TN + FP)(TN + FN)}$

We use a threshold of 0.5 in the confusion matrix to estimate our threshold dependent metrics (Pr, Re, F1, and MCC). Although prior research suggests that threshold independent metrics (AU-ROC and AU-PRC) are more accurate estimators of model performance [58], we report both to provide practitioners with more insights on how data quality antipatterns affect their specific use case. For example, in some cases, identification of True-Positives using Recall may be more important than AU-ROC or Precision. Additionally, while dealing with datasets that have class imbalance, the AU-PRC metric is a better estimator of model performance than AU-ROC.

## 4 Results

In this section, we describe the results of each of our research questions.

4.1 RQ1: What is the prevalence of data quality antipatterns in software defect prediction data?

### *Motivation.*

Despite the widespread use of SDP data in software engineering research [23, 34, 59], researchers utilizing SDP datasets lack an empirical understanding of the presence of data quality antipatterns within the software defect prediction datasets. Singular data quality antipatterns have been found in Software Engineering datasets ([2, 9, 17, 60]), however, to the best of our knowledge, no research yet checked the prevalence of multiple data quality antipatterns in the context of software engineering. Hence, in this RQ, we aim to check the prevalence of data quality antipatterns in SDP data.

Practitioners can use our research as a case study to understand the manifestation of data quality antipatterns in their datasets. In this RQ, we investigate the prevalence of data quality antipatterns in SDP data. Understanding the prevalence of these antipatterns is important for both researchers and practitioners, as it can provide valuable insights into the factors that impact the performance and interpretation of machine learning models used for defect prediction. By identifying and addressing these antipatterns, practitioners can improve the reliability and accuracy of their models, leading to more informed and effective decision-making in software engineering tasks.

**Approach.** Against each of the antipatterns discussed in Section 2, we check the prevalence of data quality antipatterns in the SDP data using the antipattern detection strategies provided in Section 3.

**Results.** We found the prevalence **Bram:** [what are top-3, how prevalent (num of instances?)] **Aadi:** [how to rank disparate items? e.g., are 2.6% duplicates more than 17% class overlap? different antipatterns seem to be uncomparable, and hence cannot be ranked] of nine anti-patterns (schema violations, class overlapping data, class imbalance, duplicated data, constant features, correlations & redundancies, tailed distribution data, unnormalized distributions, and mislabels) in the studied SDP dataset. We did not detect the presence of four antipatterns (i.e., *Data Miscoding*, *Inconsistent Representation*, *Missing Values* and *Data Drift*) in the studied datasets. **Bram:** [how common in software analytics] **Aadi:** [Null check (missing values) would be done during data collection, data miscoding is data processing error – can't be there in static data] **Bram:** [how big is the dataset.] **Aadi:** [total=73,395, and mean=2294, median=1717.5, pls also refer to 2] Since *Data Miscoding* is a dynamic issue, an ML pipeline (or non-ML data-driven program) should validate the correct data type; nevertheless, we are unable to identify this as an antipattern in the static dataset from Yatish et al [32]. Furthermore, there are neither missing values nor inconsistent representations in the studied SDP data. Below, we present each of the antipatterns prevalent in the SDP data:

#### 4.1.1 Row Feature Imbalance

**The studied SDP data does not have row feature imbalance.** Figure 2 shows the ratio of the number of rows and the number of columns. The values presented in the Figure 2 are nominal, with outliers in the project version *Camel-2.9.0* having the maximum (7,120) rows, and the project version *Jruby-1.1* having minimum (731) rows. All project versions have 65 columns.

#### 4.1.2 Schema violations

**2% of the studied SDP dataset has schema violations.** We observed violations for five (i.e., R8, R14, R15, R17, and R19 **Bram:** [discuss why

% imported data acts  
(not % imported rows within project)

not  
method  
here?

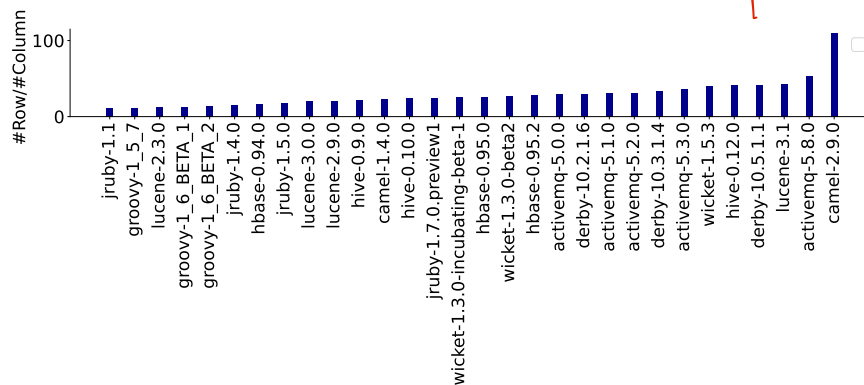

mean! then paper saying that this ratio should be 10-20 ideally?  
can we draw horizontal line for that in figure?

Fig. 2: Row feature imbalance.

probably related to size, unbalancedness, ...

these?] Aadi: [I am not sure how can I know that. The scikit tool used by Yatish et al had bugs maybe, but why specifically those, we can just speculate, not sure if we can definitely say. What do you think??] out of 20 rules defined in Table 3. A total of 30, 12, 7, 6, and 6 files had violations against rules R14, R8, R14, R15, and R17. Figure 3 shows the distribution of violations for different project versions of the studied SDP data. The maximum violations were observed for the project **hive** version 0.10.0 with 7% data having schema violations.

→ what % of projects?

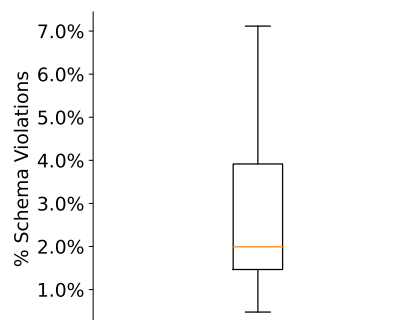

Fig. 3: Distribution of Schema violations amongst different versions of the SDP data.

#### 4.1.3 Data Distribution Anti-patterns

- **Tailed Distribution.** Across various project versions of the SDP data, 40% of the metrics were identified as tailed. The percentage of

show many %?

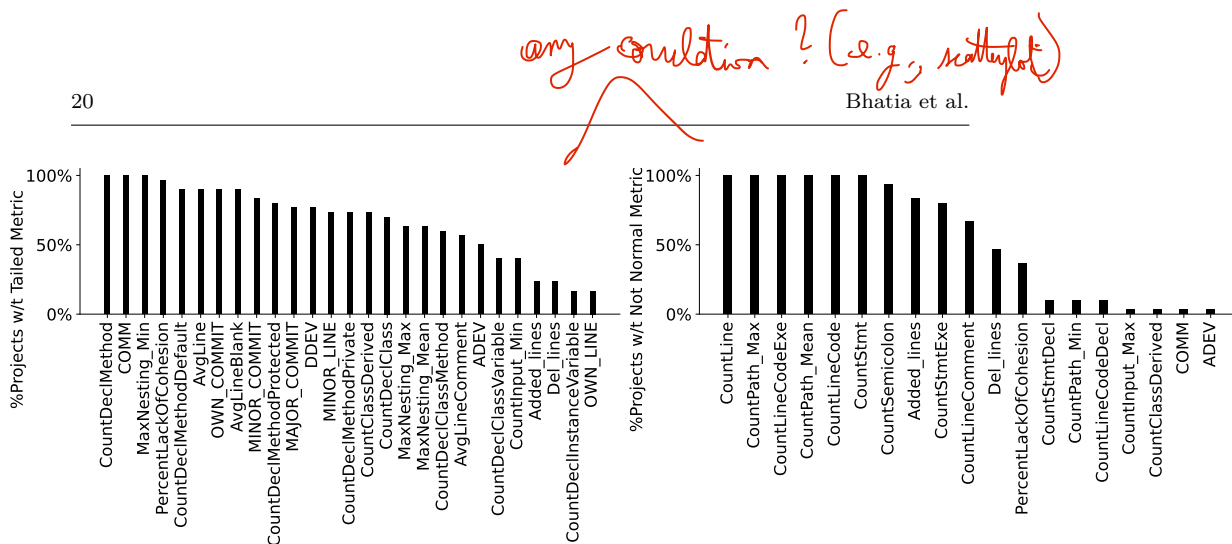

Fig. 4: *Bram: [Demographies of dataset? num rows and num projects give first?]* Aadi: [fixed in Table 2] Tailed metrics (left) along with Unnormalized metrics (right) across different project versions of the SDP data.

*Bram: [] Aadi: [some other comment, i cant undertand now.]*

projects in which a metric was identified as tailed is shown in Figure 4 (left). The metrics *CountDeclMethod*, *COMM* and *MaxNesting\_Min* are tailed across all projects.

- *Unnormalized Distributions*. **17% of metrics are consistently unnormalized, while 37% are inconsistently unnormalized.** The 19 metrics detected as unnormalized are illustrated in Figure 4 (right).
- *Constant Features*. We found that the metric, *Minor\_Commit* remained constant across five project-versions: *ActiveMQ-5.1.0*, *5.2.0*, *5.3.0*, *5.8.0* and *Derby-10.5.1.1*.
- *Data Drift*. We found no evidence of data drift between successive versions of the SDP data. Furthermore, we found no drift between the first and final versions of the same project.

#### 4.1.4 Packaging Errors: Duplicated Data

**Duplicate values are commonly prevalent in the SDP data, with a median of 2.6% data duplicated.** *Bram: [how is it commonly if its just 2.6%]* Aadi: [todo: check other papers who reported it - theres that nASA issues paper if I remember correctly.] Figure 5 depicts the percentage of duplicated rows across different project versions of the studied SDP data. The project *ActiveMQ-5.8.0* contains the maximum, i.e., 17.4% duplicates, whereas the project *Hbase-0.94.0* contains no duplicates.

#### 4.1.5 Label Antipatterns

**Class Overlap.** For the project versions of the studied SDP data, a median of 17% of data had overlapping classes. *Bram: [17=high?]* Aadi:

project versions  
or  
rows?

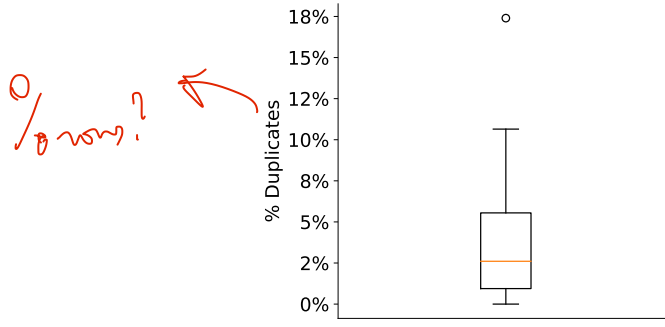

Fig. 5: Percentage of duplicated data detected in the studied SDP dataset.

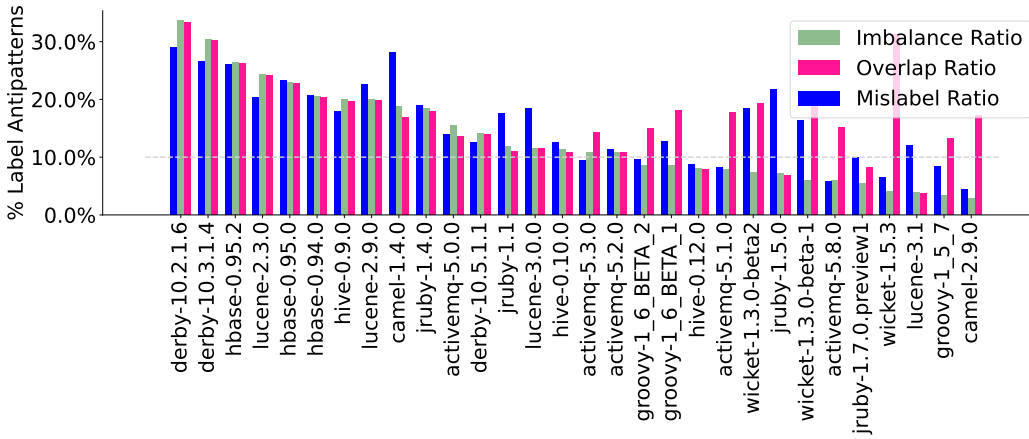

Fig. 6: Distribution of Label Antipatterns in the SDP data. We present the ratio of class imbalance, class overlap along with mislabels.

*[Literature does not specifically claim what's "high"- but such overlap percentages are expected in SDP [9, 6]].* The percentage of overlapping instances detected on a per-project version basis is shown in red Figure 6. The project Derby, version 10.2.2.6, had a highest amount of overlapped instances (i.e., 654 out of 1,963). According to prior studies, such outcomes are to be expected in defect prediction [9, 6].

*Class Imbalance.* *Bram: [do symmetric stacked barchart!] Aadi: [ symmetric bar 1) wont let me give a head-to-head comparison between all label aps 2) I wont be able to do symmetric with 3 sub-aps. Am I missing your point tho?]* **A median of 11% class imbalance is prevalent in the studied SDP dataset.** Figure 6 shows the ratio of minority classes (buggy instances) with respect to the total data size per project-version-basis. Class Imbalance is depicted by

the blue color in Figure 6. As shown in the Figure, project-versions having high class imbalance are also likely to have class overlap. Such findings are not uncommon as prior research has indicated the relation between the two antipatterns [10,11,12]. Below the threshold of 10%, as demarcated by the gray line in Figure 6, 43% of the project-versions have class imbalance. While a specific threshold for “high” class imbalance is not provided in literature, we use 10% as an arbitrary value to indicate the prevalence of class imbalance in different project-versions of the studied SDP dataset.

*Mislabeled.* There is a significant presence of mislabeling in the SDP data, as demonstrated by Yatish et al. [32]. The inconsistencies observed between the two labeling schemes are depicted in green color in Figure 6. A median of 15% of labels had conflicting labels produced from the two (i.e., *Heuristic* or *Realistic*) labeling strategies.

#### 4.1.6 Correlation & Redundancy.

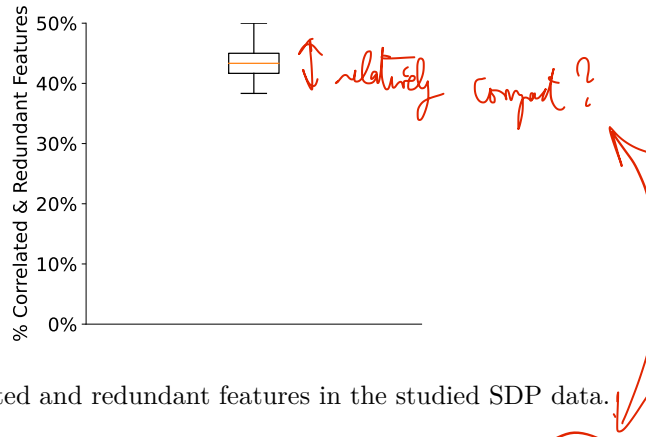

Fig. 7: Correlated and redundant features in the studied SDP data.

**The amount of correlations & redundancies are inconsistent in the SDP data. The y-axis starts from the minimum amount percentage of 38%** Figure 7 shows the distribution the percentage of correlated & redundant features within different project versions of the studied SDP dataset. A median of 43.3% metrics are correlated and redundant. This is accompanied by a high variance of 8%, which indicates that amount of correlated and redundant metrics differ in different project-versions of the studied SDP data.

#### 4.2 Overlap of Antipatterns

In the previous subsection, we studied the prevalence of different antipatterns in our studied SDP dataset. In this subsection, we present the ex-



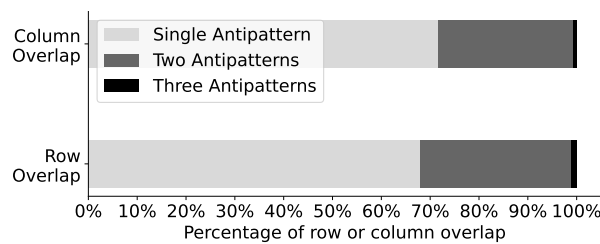

Fig. 8: Overlap between multiple antipatterns. We do not show the data points that do not have any antipattern.

tent of overlap of these antipatterns. We bifurcate the results into two categories: row-level antipatterns (including schema violations, mislabels, class overlapped rows, and duplicates) and column-level antipatterns (encompassing tailed, unnormalized, constant, and correlated & redundant features). Our focus is on overlap within the same category (i.e., row-level and column-level) due to the inherent overlap between the row and column level antipatterns.

*how much actually?*  
*should be interesting to add*

- **Row level overlap.** Majority (68%) of rows impacted by antipatterns do not exhibit any overlap. As shown in Figure 8 only 31% rows having antipatterns have two antipatterns, out of which 94% cases are overlapped with Mislabels and Class Overlap. *Bram: [any idea why these? is this good news? bad news?]. Aadi: [we explore the effects of these in the subsequent rqs and point back to this finding as the motivation for subsequent rqs.]* The remaining 1% cases having row-based antipatterns had three antipatterns affecting the same row.
- **Column level overlap.** Most (72%) columns having antipatterns do not have any overlap with another antipattern. 90% of the remaining 28% cases with two column-based antipatterns comprised correlation & redundancy along with tailed features. A trivial amount of columns (0.4%) columns had three antipatterns.

*Aadi: [say here that in the next section, we study the impact of this overlap.]* As shown in Figure 8, 71.6% columns and 67.9% rows have a single antipattern.

### Summary of RQ1

Anti-patterns in the SDP data include *schema violations*, *correlated & redundant features*, *distribution antipatterns* (tailed, constant, and un-normalized distributions), *labeling antipatterns* (mislabeling, class overlap, class imbalance and duplicated data). We found no instances of *data miscoding*, *missing values* or the *data drift* antipattern. For antipatterns having overlap on a row-level, 94% cases comprise of mislabels and class overlap. For the column-level antipattern overlap, 90% cases include correlated & redundant features along with tailed features.

4.3 RQ2: Does the order of cleaning data quality antipatterns impact the model performance?

**Motivation.** The data pre-processing phase in ML pipelines involves preparing the data for training the ML model, as noted by Amershi et al. [27]. This includes cleaning, performing transformations, and more, a topic that has been widely studied in literature and is outlined in our Section 2. However, despite the recognition of the importance of cleaning data quality antipatterns, the optimal order for addressing multiple antipatterns remains unknown. Understanding the influence of the order in which antipatterns are cleaned is crucial, as it can affect the size of the training data and, thereby, the performance of the ML model. As demonstrated in our previous research question, data quality antipatterns often coexist, exacerbating this need. The overlap of these antipatterns may potentially lead to compounded errors and biases in the dataset, and addressing them in an improper sequence may inadvertently amplify these issues, or negate the benefits of cleaning performed in previous steps. For instance, normalizing data before addressing missing values might lead to skewed distributions, impacting the accuracy of imputation techniques. Conversely, handling class-overlapped rows prior to normalization could remove valuable data points that are actually significant once the data is scaled appropriately. Therefore, establishing an effective order for cleaning operations is essential to ensure that each step enhances the quality of the data without introducing new issues or magnifying existing ones.

**Approach.** We remove antipatterns in different orders from the training data and build ML models using the studied learners. An overview of this process is shown in Figure ??.

We categorize the cleaning into four groups: *Filtering* (Fi), *Transformations* (Tr), *Class Overlap* (Ov), and *Mislabeling* (Mi). This classification into these groups is based on the type of cleaning required for each antipattern. *Bram: [citations?] Aadi: [This was our choice of design based on logic, eg, rows having violations "should" be bad, so we we ought to remove them. class overlapped rows "should" be removed since learner gets confused on these.]* For instance, the *Fi* category involves filtering schema violations, duplicated data,

repeat % here

constant features, and correlated and redundant features, as data is removed from rows or columns. The *Tr* category entails performing log-transformation and z-scoring to transform tailed and unnormalized features respectively. The *Mi* cleaning category includes mislabel correction. Finally, the *Ov* category removes overlapping classes. We keep *Class Overlap* separate from other filtering-based cleanings because *Mislabeling* explicitly impacts *Class Overlap*, while having no effect on other cleaning techniques, such as schema violations or constant features.

Next, we create permutations of the four cleaning types to access the impact of order of cleaning. From all the permutations, we exclude the permutations that lead to the same result. In particular, the positioning of *Mi* at any step before *Ov* does not matter, as both *Mi* and *Ov* are based on the response (y-label) and do not impact the explanatory variables. For instance, in the case of *FiTrMiOv*, mislabel positioning before overlap (i.e. *FiMiTrOv*, or *MiFiTrOv*) yields the same data. Similarly, mislabel correction after class overlapping (i.e., *OvFiTrMi*, *OvFiMiTr*, *OvMiFiTr*) yields the same data as well. Overall, we obtain 12 permutations of *Fi*, *Tr*, *Mi*, and *Ov*, out of their 24 permutations, which we refer to as cleaning **orders** henceforth. These cleaning orders are: *FiMiOvTr*, *FiOvMiTr*, *FiTrMiOv*, *FiTrOvMi*, *MiOvFiTr*, *OvMiFiTr*, *MiOvTrFi*, *OvMiTrFi*, *TrFiMiOv*, *TrFiOvMi*, *TrMiOvFi*, and *TrOvMiFi*. We clean the training data based on each of these orders, and build an ML model using the model-building process outlined in Section 3. Using the unseen test set, we obtain Precision, Recall, F1, MCC, AU-ROC, and AU-PRC from each model.

In this RQ, our objective is to check for the order sequences which may potentially lead to an impact in the model performance. To study this, we repeatedly divide the 12 orders into two groups based on the occurrence of an antipattern pair - one group with a considered antipattern preceding another, and the other group with the antipattern following another. For instance to check whether Filtering should be performed before or after performing Transformation, we form the sub-sequence  $Fi \rightarrow Tr$  along with its inverse sub-sequence  $Tr \rightarrow Fi$ . The the sub-sequence  $Fi \rightarrow Tr$  has six orders in which Filtering is performed before Transformation (i.e., *FiMiOvTr*, *FiOvMiTr*, *FiTrMiOv*, *FiTrOvMi*, *MiOvFiTr*, *OvMiFiTr*), while its inverse sub-sequence,  $Tr \rightarrow Fi$  has the remaining six orders. We compute the frequency of the orders with a particular sub-sequence outperforms its inverse sub-sequence. To enable fairness, we compare the performances of models built from different cleaning orders of the same training data. This is done by checking the top performing orders of a particular training data split from the 10-folds of randomized training-testing splits. For instance, while checking whether the sub-sequence  $Fi \rightarrow Tr$  outperforms its inverse, for a given training dataset, we check whether the orders having the top 50 percentile performance belong to the  $Fi \rightarrow Tr$  sub-sequence or its inverse sub-sequence  $Tr \rightarrow Fi$ . If there is a tie, then we add weights to both the inverse sub-sequence and the sub-sequence. *Bram:* [why?] *Aadi:* [if win rate of both sequence and inverse sub sequence is 50% then we add equal weights to both to make weightage work.] We repeat the process for all performance met-

Complicated explanation  $\rightarrow$  use figure?

Table 5: sub-sequence win ratio over its inverse sub-sequence. We do not study cases of  $Mi$  with  $Tr$  or  $Fi$  since Mislabel correction has no impact of the two.

| Learner | sub-sequence | F1   | Precision | Recall | MCC  | AU-ROC | AU-PRC |
|---------|--------------|------|-----------|--------|------|--------|--------|
| Rf      | MiOv         | 61.3 | 38.5      | 64.4   | 53.2 | 38.6   | 62.3   |
| Xgb     |              | 56.1 | 29.8      | 62.8   | 51.1 | 39.5   | 59.7   |
| Lr      |              | 60   | 60.4      | 59.5   | 65.1 | 56.5   | 66.1   |
| Dnn     |              | 55.6 | 55.4      | 56     | 54.7 | 46.1   | 59.3   |
| Rf      | FiTr         | 54.2 | 51.9      | 60.7   | 52.2 | 48.4   | 52.5   |
| Xgb     |              | 50.7 | 46        | 57     | 45.9 | 53.7   | 49.7   |
| Lr      |              | 58.2 | 53.6      | 61.2   | 54.4 | 49.2   | 50.7   |
| Dnn     |              | 48   | 47.9      | 52.7   | 48.2 | 50.6   | 50.1   |
| Rf      | TrOv         | 62.3 | 65.6      | 63.6   | 64.7 | 46.1   | 49.3   |
| Xgb     |              | 67.6 | 59.2      | 67.7   | 66.7 | 43.8   | 52.8   |
| Lr      |              | 52   | 53.9      | 62.6   | 55.5 | 45     | 57.9   |
| Dnn     |              | 56.2 | 49.9      | 56.5   | 54.1 | 47.6   | 53.7   |
| Rf      | FiOv         | 61.9 | 62.1      | 68.4   | 59.6 | 45     | 49.8   |
| Xgb     |              | 61.9 | 52.1      | 69.9   | 56.5 | 51.2   | 48.1   |
| Lr      |              | 58.5 | 51.8      | 69.1   | 59.8 | 47     | 61.6   |
| Dnn     |              | 51.4 | 45.4      | 55.9   | 50.5 | 49.9   | 55.7   |

rics (Recall, F1, MCC, AU-ROC, and AU-PRC) to evaluate the percentage of a particular sub-sequence winning over its inverse.

#### Results.

No sub-sequence achieves a high win rate *Bram:* [still quite high!] *Aadi:* [yes, but no "clear" win for us to draw a phenomenon from. Even the win rates seem arbitrary with no discernable pattern.] (greater than 70%) over its inverse sub-sequence. The win rates of various sub-sequences over their inverse sub-sequences are shown in Table 5. For instance the win rate for a sub-sequence MiOv for random forest learner's AU-PRC is 62.3, and sub-sequently the win rate of the inverse sub-sequence, i.e., OvMi will be 37.7. Most sub-sequences (95th percentile) have win rates below 55%, suggesting that the sub-sequence orders perform better randomly<sup>7</sup> compared to their inverse sub-sequences.

Although some sub-sequences win against their inverse sub-sequences, the win rates are trivial, i.e., below 70%. The observed win rates depend on the classifier or metric used. For example, the maximum win rate of 70% is obtained for the sub-sequence  $Mi \rightarrow Ov$  over its inverse,  $Ov \rightarrow Mi$ , when considering the precision of the XGBoost classifier. However, for the same precision metric, the other classifiers (RF, LR, and DNN) show win rates for  $Mi \rightarrow Ov$  close to 50% (i.e., 39%, 60%, and 55%, respectively). *Bram:* [Also can you do median across learners in the table to control for this?] *Aadi:* [please find in table: 6 Still can't find any discernable pattern. Perhaps 1) auc is most resilient among other metrics. 2) altho the numebrs are not very authoritative, the Mi Ov seems to have higher win rates as compared to its opp. This makes sense because Ov then Mi correction means Cls Ov was done based on

<sup>7</sup> A win rate of 50% represents an equal likelihood of the sub-sequence outperforming its inverse or vice versa.

maybe  $N=15$ ? do we have  
 $\uparrow$  3 equally-sized subsets?  
 we need 3 cases:  $< 50-N\%$   
 $\geq 50-N\%$   
 and  
 $\leq 50+N\%$   
 $> 50+N\%$   
 (and  $> 65\%$ ? otherwise difference gain significant)

how is this threshold determined?

more in Table 5

| Subsequence | auc  | auprac | f1   | mcc  | precision | recall |
|-------------|------|--------|------|------|-----------|--------|
| FiOv        | 47.0 | 61.6   | 58.5 | 59.8 | 51.8      | 69.1   |
| FiTr        | 49.2 | 50.7   | 58.2 | 54.4 | 53.6      | 61.2   |
| MiOv        | 56.5 | 66.1   | 60.0 | 65.1 | 60.4      | 59.5   |
| TrOv        | 45.0 | 57.9   | 52.0 | 55.5 | 53.9      | 62.6   |

Table 6: *Aadi: [this is temp table to take learner discrepancies into account.]*

*incorrect knowledge of labels* These values demonstrate the negligible impact of applying mislabel correction before or after class overlap correction for the precision metric. Similar results are found for other metrics, such as Recall, F1, MCC, AU-ROC, and AU-PRC, as shown in Table 5.

Table 5 also presents the win rates for other sub-sequences, including  $Fi \rightarrow Tr$ , which examines the impact of filtering before (or after, as the “inverse sub-sequence”) transformation;  $Tr \rightarrow Ov$ , which investigates the effect of transformation prior to overlap correction; and  $Fi \rightarrow Ov$ , which assesses the impact of filtering before overlap correction.

Metrics such as AU-PRC, AU-ROC, Precision, and F1 show win rates close to 50%, while *Recall* exhibits comparatively higher win rates for all sub-sequences. In fact, the highest win rates include a 61% win rate for  $Fi \rightarrow Tr$ , a 67% win rate for  $Tr \rightarrow Ov$  using the XGBoost classifier, and a 69% win rate for  $Fi \rightarrow Ov$  when considering recall.

#### Summary of RQ2

Order of cleaning antipatterns has no impact on the performance of the defect prediction models. The likelihood of a given order outperforming its inverse order is close to 50%, which is random chance. The maximum win rates obtained by a given sub-sequence over its inverse are based on the studied learner and are trivial (less than 70%).

#### 4.4 RQ3: How do data quality anti-patterns impact model performance?

does not match motivation?

##### **Motivation.**

The impact of removal of one antipattern on the other antipatterns is not known. It is important to understand this relationship, as multiple antipatterns coexist in the data, as evidenced by our **RQ1** findings. While prior studies [9, 2, 32, 14] have presented the impact of the prevalence of an antipattern on model performance when other antipatterns are present, it is unclear what the impact of the prevalence of an antipattern is when the other antipatterns have been cleaned out. Understanding this relationship is important because in practical scenarios, multiple antipatterns are present which may have overlapping effects. This raises the question of whether fixing an antipattern is necessary when other antipatterns have been removed, given the high cost of

removal. For instance, overlap removal removes a high proportion of data (as evidenced by a median of 17% data removed on a row level in **RQ1**). Similarly, on a column level, removing correlated & redundant features leads to a data loss of a median of 43% of features. Indeed, noisy data can still contribute valuable information to ML models, particularly when clean data is scarce or unavailable [61,62,63]. Hence, to obtain the value in removing a specific antipattern, it is important to assess the impact singular particular antipattern in a scenario where all the remaining antipatterns are removed.

**Approach.** The goal of this research question is to evaluate the impact of various antipatterns on the performance of machine learning (ML) models. To achieve this, we introduce individual antipatterns one-by-one into an “all-clean” dataset and check for any significant performance differences caused by that antipattern. While one could argue for cleaning an antipattern from an “all-dirty” dataset, we adopt the former approach to specifically understand the impact of each antipattern rather than evaluating a cleaning technique. To accomplish this, we begin by creating a clean dataset in which all antipatterns are removed with the *FTMO* order. Next, we add back one antipattern at a time and build ML models to assess performance changes caused by a specific antipattern. Figure 9 illustrates this approach. A detailed explanation of the data and model preparation process is provided below.

1. *Generation of a baseline of “clean” set.* For each version of the project, we split the data into training (80%) and testing (20%) sets. We clean the training data of all antipatterns to generate an “all-clean” set, which is devoid of any antipattern. In **RQ2**, we found that there is no clear order that has a significant impact on the model performance. Therefore, we devised our own rationale for selecting an order from the different orders mentioned in **RQ2**. Specifically, we chose the order *FTMO* (i.e., *Filter* → *Transform* → *Mislabel* → *Overlap*) based on the following rationale:
  - Cleaning schema violations involve rule-based unit testing based on thresholds. Such thresholds cannot be put in place once transformations like z-scoring and logging have been done. Hence, *filtering should be performed before transformation*.
  - Moreover, if a certain feature will be eliminated as a correlated or redundant feature, it doesn’t make sense to transform that feature. As a result, *filtering should be performed before transformation*.
  - Class overlap should have mislabel correction applied to ensure that the class overlap detection has accurate knowledge of the response label. Hence, *class overlap should be performed after mislabel correction*.
  - To ensure that the data distribution available for detection of overlapping classes is the same as that used for model training, *class overlap should be carried out at the end*.
2. *Adding back antipatterns.* To assess the impact of each antipattern, we add them back into the clean data. In particular, we add rows with schema violations, duplicates, and class overlap to assess their impacts. Similarly, the column-based antipatterns (correlated and redundant features, and con-

for  $\pm 70\%$  of cases, the all-dirty dataset == dataset with 1 antipattern? see RQ1?

not same motivation?

isn't that the same, since clean data obtained by cleaning all-dirty? see...

order seems to matter conceptually? or just confusing

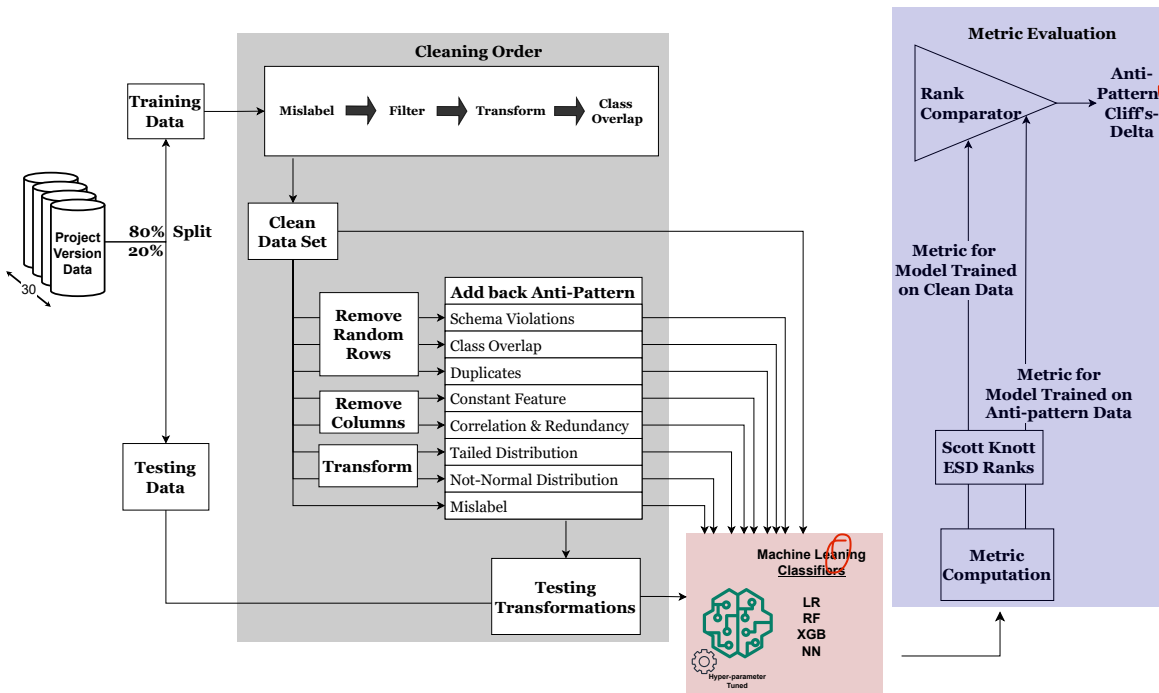

Fig. 9: Approach for assessing the impact of different data quality antipatterns.

*Bram:* [the "remove random rows, columns and transform-> is this because size is the same?]  
*Aadi:* [yes, this is to keep size consistent.]

stant features) are added as additional columns while assessing their impacts. We do not perform the transformation-based corrections (i.e., log or z-transformations) for a feature which is tailed or non-normal respectively to analyze the impact of the two antipatterns.

As previous research suggests that model performance depends on data size [1, 64], to eliminate bias, we control for the data size by maintaining a consistent size across all training datasets while adding antipatterns back. We randomly remove clean data while adding back each antipattern to maintain the same size as the clean set. For example, when adding back schema violations, we first add the  $k$  violations back into the clean dataset and then randomly remove  $k$  rows to keep the size consistent. We repeat this process for each filter-based antipattern along with class overlap.

3. *Model generation and metric evaluation.* We build machine learning models for four learners using the settings described in Section 3. We generate F1, Precision, Recall, MCC, AU-ROC, and AU-PRC metrics on the unseen test set. Since ML pipelines use the same preprocessing components for training and testing infrastructures [27, 65], we perform the same transformations on the training set as that of the training set. We use the Scott-Knott ESD [66]

*could bias analysis, i.e., not just impact of anti-pattern, also of removed data points?*



not to other antipatterns' results?

ranking algorithm to compare the metrics of the antipattern-containing sets to the clean set and determine if there is a statistically significant difference. The ESD test is an effect-aware variant of the traditional Scott Knott test, which uses hierarchical clustering to partition different sets of data means into statistically distinct groups. We adopt the values of  $\alpha = 0.05$  from prior research [66]. For each project-version of the SDP data, we evaluate 10 trained models using various metrics. Each metric is evaluated on different performance groups, including *tailed*, *unnormalized*, *constant feature*, *duplicates*, *schema*, *correlation & redundancy*, *mislabel*, *class overlap*, and a *clean* set. We use the Scott-Knott method to form statistically significant ranking groups for each metric. If an antipattern has a different rank as compared to the clean set, we consider it to be statistically significant. For each significant comparison, we also calculate the effect size.

4. *Effect size for significant comparisons.* We use Cliff's  $\delta$  [67] as a measure of effect size to compare two groups of scores and determine their difference magnitude. Ranging from -1 to 1, a strong effect size is indicated by values close to 1 and no or negligible effect size by values close to 0. Cliff's  $\delta$  is preferred over traditional measures such as Cohen's  $d$ , as it is more robust and insensitive to sample size, making it suitable for small sample sizes. We present the rank difference ( $R \delta$ ) and Cliff's  $\delta$  with respect to the clean set, with negative values indicating improvement from the clean set. We use the following interpretation of Cliff's  $\delta$  [67].

$$\text{Cliff's } \delta \text{ Effect Size} = \begin{cases} \text{Negligible,} & \text{if } |\delta| \leq 0.147 \\ \text{Small,} & \text{if } 0.147 < |\delta| \leq 0.33 \\ \text{Medium,} & \text{if } 0.33 < |\delta| \leq 0.47 \\ \text{Large} & \text{if } |\delta| > 0.474 \end{cases}$$

**Results.** Five antipatterns *Tailed*, *Mislabel*, *Class Overlap*, *Class Imbalance*, *correlation & redundancy* have a statistically significant effect on the performance metrics; however, most antipatterns introduce only a small to medium boost/reduction of performance of ML models as indicated by the small to medium effect size. Table 7<sup>8</sup> 9 10 shows addition of antipatterns<sup>11</sup> that have a statistically significant comparisons to the clean set, as indicated by a different ranking of the Scott Knott ESD test.

**Different antipatterns have different impacts on different performance metrics.** However, only the *Tailed* and *Class Overlap* antipatterns have a medium or large effect size for some performance metrics. The *Class*

<sup>8</sup> “N”, “S”, “M” and “L” indicate negligible, small, medium, and large effect sizes respectively. The numerical value is provided next to the interpretation.

<sup>9</sup> Antipatterns having medium and large effect sizes are bolded.

<sup>10</sup> Negative sign shows increase in model performance after the introduction of that antipattern in the clean set.

<sup>11</sup> Abbreviations used: “Cls” for “Class”, “Ovr” for “Overlap”, “Imb” for “Imbalance”, “Cor Rdn” for Correlation & Redundancy, and “Unnrm” for “Unnormalized”

lit confounding

→ should data with 1 antipattern also be compared to original dirty dataset?

Table 7: Statistically Significant Metrics for all four learners. Abbreviations “R  $\delta$ ” is used for rank difference w.r.t. the clean set, “Effect” for Cliff’s  $\delta$  Effect Size, and “AP” for the Antipattern that is added to the clean set.

|           | Neural Network |            |                 | Logistic regression |            |                  | Random Forest |            |                 | Xg Boost |            |                 |
|-----------|----------------|------------|-----------------|---------------------|------------|------------------|---------------|------------|-----------------|----------|------------|-----------------|
| Metric    | AP             | R $\delta$ | Effect          | AP                  | R $\delta$ | Effect           | AP            | R $\delta$ | Effect          | AP       | R $\delta$ | Effect          |
| Precision | Tailed         | 1          | S(-0.31)        | Tailed              | 2          | <b>L (-0.48)</b> | Cls Ovr       | -1         | S(0.17)         | Cls Ovr  | -1         | S(0.18)         |
| Recall    | Tailed         | 2          | <b>L(-0.52)</b> | Unnrm               | 1          | N(-0.06)         | Cls Ovr       | 1          | <b>M(-0.35)</b> | Tailed   | 1          | N(-0.13)        |
|           | Mislabel       | -1         | S(0.2)          | Mislabel            | -1         | S(0.16)          |               |            |                 | Nt Nrm   | 1          | N(-0.13)        |
|           | Cls Ovr        | 1          | N(-0.11)        | Cls Ovr             | 1          | N(-0.14)         |               |            |                 | Cor Rdn  | 1          | N(-0.1)         |
|           | Cls Imb        | 1          | S(-0.19)        | Cls Ovr             | 1          | N(-0.14)         |               |            |                 | Cls Ovr  | 2          | S(-0.33)        |
| F1        | Tailed         | 1          | S(-0.33)        | Tailed              | 1          | <b>M(-0.33)</b>  |               |            |                 | Cor Rdn  | -1         | N(0.1)          |
|           | Cls Imb        | 1          | S(-0.18)        | Cor Rdn             | -1         | N(0.07)          |               |            |                 | Mislabel | -1         | N(0.09)         |
|           |                |            |                 | Mislabel            | -1         | N(0.1)           |               |            |                 |          |            |                 |
|           |                |            |                 | Cls Ovr             | -1         | S(0.19)          |               |            |                 |          |            |                 |
| MCC       | Tailed         | 1          | <b>M(-0.39)</b> | Tailed              | 1          | <b>M(-0.43)</b>  | Cls Ovr       | -1         | S(0.2)          | Cor Rdn  | -1         | S(0.16)         |
|           | Cor Rdn        | -1         | S(0.2)          | Cls Ovr             | -1         | S(0.31)          |               |            |                 | Cls Ovr  | -2         | S(0.3)          |
|           | Cls Ovr        | -1         | S(0.22)         |                     |            |                  |               |            |                 |          |            |                 |
| AU-PRC    | Tailed         | 1          | S(-0.16)        | Nt Nrm              | 1          | N(-0.12)         | Tailed        | 1          | N(-0.14)        |          |            |                 |
|           | Cor Rdn        | -1         | S(0.17)         | Cls Ovr             | 1          | S(-0.2)          | Cor Rdn       | 1          | N(-0.12)        |          |            |                 |
|           | Cls Imb        | 1          | N(-0.14)        |                     |            |                  | Mislabel      | 1          | N(-0.11)        |          |            |                 |
|           |                |            |                 |                     |            |                  | Cls Ovr       | 1          | S(-0.16)        |          |            |                 |
| AU-ROC    | Tailed         | -1         | S(0.17)         | Tailed              | -1         | S(0.31)          | Cor Rdn       | -1         | S(0.27)         | Mislabel | -1         | N(0.12)         |
|           | Cor Rdn        | 1          | N(-0.12)        | Cls Ovr             | 1          | <b>M(-0.47)</b>  | Cls Ovr       | 1          | <b>M(-0.44)</b> | Cls Ovr  | 1          | <b>M(-0.36)</b> |
|           | Cls Ovr        | 2          | S(-0.3)         |                     |            |                  |               |            |                 |          |            |                 |
|           | Cls Imb        | -1         | N(0.13)         |                     |            |                  |               |            |                 |          |            |                 |

**Overlap antipattern has a statistically significant impact on multiple metrics with a small to large effect size.** Along with the AU-ROC metric, that has a medium effect size for three out of the four studied learners, class overlap impacts recall with medium to large effect size for two learners (NN and RF), medium effect on MCC for two learners (NN and LR), along with a small effect on the precision of RF and XGB. *Bram: [tailed and clas overlap only these lead to M or L (and negative)? -not clear?]* *Aadi: [updated.]* A negative effect size indicates that introducing the specific antipattern increase the model performance. Particularly, all four learners observe a boost in performance with class overlapped rows introduced into the dataset. Similarly, **introduction of Tailed distributions impact the model performance metrics with a small to medium effect sizes**; however, this impact is metric-dependent as shown in the Table 7. Other antipatterns like unnormalized distributions<sup>12</sup>, schema violations, and duplicates. Interestingly, the mislabel antipattern had no effect on any performance metric except for Recall for NN and LR. We check the reasons for such a result in Section 8.

On the learner level, only the NN learner is impacted by class imbalance with a small effect size. The XGB learner is impacted by the least antipatterns

<sup>12</sup> While NN has an impact on the recall metric, the effect size is negligible

*- incomplete sentence*

(only Class Overlap and correlation & redundancy), while other antipatterns have a negligible effect. Moreover, only the LR learner is impacted by Unnormalized features, however, the effect size is negligible.

*Bram: [how (un) stable are results across learners? this could be a finding!]*  
*Aadi: [Added.]* Furthermore, on the learner level most learners assign the first SK rank to the class overlap along different metrics, indicating that all learners are in agreement that class overlap rows impact the all learner's performance the most. Particularly, the learner's aggregated agreement on SKranks along different metrics for Class Overlap is 0.75; tailed is 0.79; constant feature, the clean set, schema violations, and package antipatterns is 0.62; class imbalance and un-normal is 0.58; correlation & redundancy is 0.54; and mislabel is the least of 0.5. Along with the results presented in Table 7, this indicates that different antipatterns have different impact on the model performance.

On a metric level, only the MCC for NN and XGB are impacted by Correlations & Redundancies. Similarly, Mislabel impacts only the recall metric (while other effects are negligible). Finally, F1 is impacted by the least antipattern<sup>13</sup>.

#### Summary of RQ3

Although five antipatterns (*Tailed*, *Mislabel*, *Class Overlap*, *Class Imbalance*, *Correlation & redundancy*) have a statistically significant effect on performance metrics, most antipatterns only introduce a negligible to small effect. Among them, only the Tailed and Class Overlap antipatterns result in a medium or large effect on some of the model performance metrics.

RQ4: Do models built from different antipatterns give consistent interpretation results?

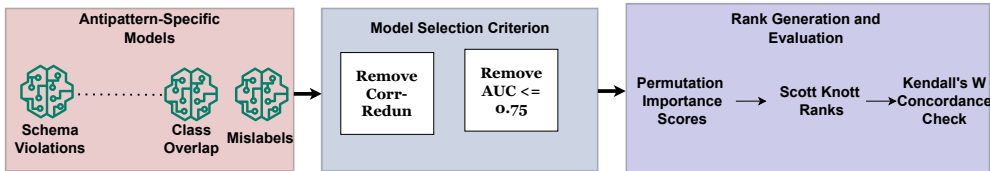

Fig. 10: Methodology to check concordance between different antipattern-specific models.

**Motivation.** Interpretation of ML models is essential in various organizational tasks, such as defect prediction, to avoid misguided decisions. While

<sup>13</sup> Most antipatterns have negligible effect size.

interpretation remains a significant area of research, current research primarily focuses on the model-perspective, including the impact of model performance [35], and the choice of learners [68]. However, the influence of data quality on interpretation consistency has not been explored.

This research question aims to investigate the impact of antipatterns on interpretation consistency, thereby improving our understanding of the relationship between data quality antipatterns and the reliability of interpretation outcomes obtained from ML models.

**Approach.** To check whether interpretation ranks from different antipatterns are consistent, first select ML models from different antipatterns, and then use permutation importance scores to calculate the feature importance obtained from each antipattern-specific model. Finally, we measure the concordance between the interpretation ranks. We illustrate an overview of this methodology Figure 10, and provide the details below:

- **Selection of ML models.** We use the ML models created for **RQ2**, each containing one antipattern at a time. Only models with AU-ROC  $\geq 0.75$  are considered, as models with lower AU-ROCs produce inconsistent interpretation results [69,35]. The threshold of 0.75 is also used by Lyu et al. [69] for predicting failures in job and hard drives. Moreover, we exclude the Correlation & Redundancy antipattern from our analysis, as interpretation results from models with correlated & redundant metrics are unreliable [35]. *Bram: [are they here?] Aadi: [no, we exclude in this RQ]*
- **Generating Interpretation Scores.** From the models selected in the previous step, we extract the important features learned by that model using permutation importance [70]. This study adopts a model-level interpretation approach, as opposed to instance-level interpretation.
- **Generating Feature Importance Ranks.** The model interpretation is computed on a per-project-version-level and per-learner to account for inconsistencies in interpretation across different project versions and learners [69].  
For each learner, we rank the permutation importance scores from models of each project-version to compute a feature importance rank. We use the Scott Knott ESD ranking algorithm for this purpose.
- **Evaluation of concordance.** Kendall’s W is a non-parametric measure of inter-rater agreement and consistency, particularly in cases where there are multiple raters (i.e., ML models built from the eight antipatterns along with the clean set in our case). It takes into account the agreement among all raters, rather than just comparing pairs of raters or measures, making it a more comprehensive measure of agreement. This metric was also adopted by Lyu et al. [69] to determine the consistency of interpretation rankings from different learners. For our study, we calculate the consistency of interpretation ranks from different antipatterns of the same project-version and present this concordance for each of the four learners. It ranges from -1 to 1, with values close to 1 indicating a strong positive association, values close to -1 indicating a strong negative association, and values close to 0

indicating no association. The Kendall's  $W$  interpretation is as follows:

$$\text{Kendall's } W \text{ Concordance} = \begin{cases} \text{Weak,} & \text{if } |W| \leq 0.3 \\ \text{Moderate,} & \text{if } 0.3 < |W| \leq 0.6 \\ \text{Strong} & \text{if } |W| > 0.6 \end{cases}$$

For our study, we calculate the consistency of interpretation ranks from different antipatterns of the same project-version, and present this concordance for each of the four learners.

### Results.

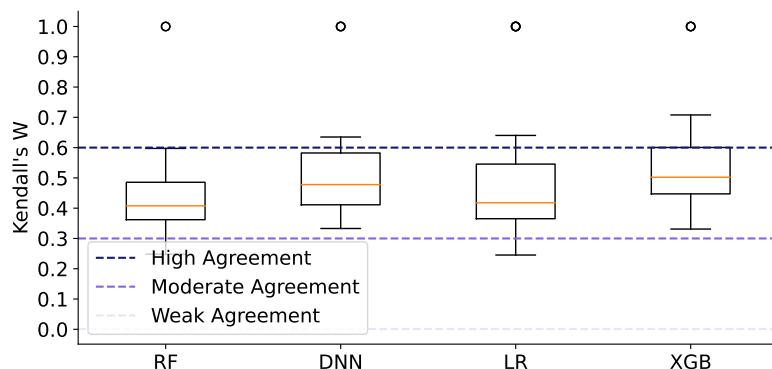

Fig. 11: Kendall's  $W$  concordance for Interpretation Ranks from multiple antipatterns.

**Interpretations from models with different antipatterns show moderate consistency.** Figure 12 displays the concordance of interpretation ranks *Bram: [which one agrees the most with the 100% clean model>?] Aadi: [I dont think we can't say that clean set interpretation ranks are 'correct' for us to be able to have this comparison, although I have added the concordance results in a temp figure ?? as per your request. The median concordance is less than 0.6 mark for all antipatterns showing that the aps moderately impact the interpretation results.]* among various antipattern-specific models for each project version. For all learners, the median concordance falls between the 0.6 and 0.3 marks, as depicted in the figure. This result suggests that there is a moderate level of agreement in the interpretation ranks across models with different antipatterns. *dimy fig. 12 here*

#### Summary of RQ3

The consistency of interpretation ranks across models with different antipatterns is moderate.

*what does this mean?  
i.e., should anti-  
patterns be removed now  
or does not matter?*

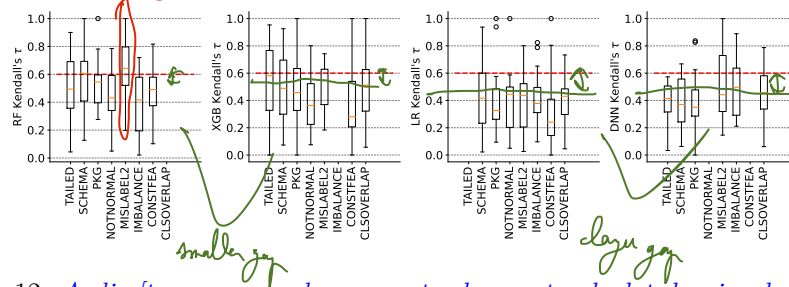

Fig. 12: *Aadi: [temp: concordance w.r.t. clean set calculated using kendal's Tau.]*

## 5 Threats to Validity

*Gopi: [I havent checked this yet]*

### 5.1 Threats to External Validity

In this study, we evaluated the performance of four learners on the SDP dataset. Firstly, our findings may have limited generalizability based on our used SDP datasets and learners. To minimize this threat for learners, we selected the learners that are widely used in defect prediction research and represent a diverse range of families [58].

In RQ2 and RQ3, we built models using the Sklearn version 1.1.3 and evaluated the impact of different antipatterns on their performance. However, we did not explore the use of other popular AI development frameworks such as R, C++, or Java.

*+ other analytics models than SL*

### 5.2 Threats to Internal Validity

In **RQ3**, we examine the effect of a specific antipattern by introducing it to the clean dataset. This experiment design allows us to evaluate the impact of the antipattern. An alternative experiment design where all antipatterns are added and then one is removed could have been conducted. However, the outcome of such an experiment would reveal the impact of “cleaning” the antipattern, rather than the antipattern itself.

Moreover, in **RQ4**, the choice of AU-ROC threshold (0.75) may impact our results. Although a high AU-ROC threshold is necessary to evaluate the impact inconsistency caused by low-performing models [69, 35].

*by tail*

### 5.3 Threats to Construct Validity

For **RQ2** and **RQ3**, we conduct the model training process 10 times for each learner for each order/antipattern. While other studies have utilized a higher number of repetitions to broaden the number of randomly sampled data splits, the sheer number of AI models generated in this research is substantial. A total of *Bram: [was not clear from methodology]*  $12(\text{orders}) * 4(\text{learners}) * 30(\text{project} - \text{versions}) * 10(\text{runs}) = 14,400$  models were generated for **RQ2** and  $10(\text{antipatterns}) * 4(\text{learners}) * 30(\text{project} - \text{versions}) * 10(\text{runs}) = 12,000$  models were generated for **RQ3**, resulting in a grand total of 26,400 models. All models are generated using hyperparameter tuning, adding to additional computational load. Despite the use of high-performance computing resources (on a server machine with 80 CPU cores), the sheer volume of AI models generated resulted in a substantial computing time of over 48 hours.

Additionally, while prior research [52] has indicated that random search is superior to other optimization techniques such as grid search, we cannot guarantee that our set of extracted hyperparameters are the most optimal.

To gauge the consistency of interpretation in **RQ4**, the use of permutation importance as the sole feature importance measure may not capture the full complexity of model interpretation. Future research may wish to employ alternative feature importance measures, such as LIME [71] or SHAP, could provide a more comprehensive understanding of the relationship between antipatterns and interpretation consistency. Moreover, in **RQ4**, we utilize the Kendall's W metric. research [35,68] dealing with low features have used metrics like Top-N score, we believe Kendall's W metric provides the most appropriate concordance results due to a high feature count in our SDP dataset, since we cannot make a pair-wise comparison while comparing interpretation results from nine raters (eight antipatterns-specific models one clean set model).

## 6 Literature Review

While in Section 2, we provided literature on data quality *antipatterns*, in this section, we discuss research in data quality along the aspects of software engineering/SDP, data quality issues in other domains, and data quality tools.

1. **Data Quality in Software Engineering and Software Defect Prediction.** In 2013, Kamei et al. [42] focused on identifying defect-prone ("risky") software changes instead of files or packages as "Just-In-Time Quality Assurance". From the perspective of data quality, this is label identification for SDP. Similarly, Zimmermann et al. [72] used labels from one project to leverage them for another project, i.e., cross project defect prediction along with the factors affecting the success of cross-project predictions were identified. In 2020, Jain et al.[73] presented an overview of data quality for machine learning applications. Jain et al. surveyed important data quality issues discussed in literature and quality management strategies at IBM. Similarly, in 2021, Gupta et



al.[74] from IBM presented a tutorial for maintaining data quality for ML tasks intended for data scientists, stewards, and practitioners. Renggli et al.[75] from Microsoft Research presented a data quality view of MLOps, specifically providing guidelines and perspectives on designing an efficient MLOps pipeline. Abdallah et al.[76] uncovered data quality issues for big data, presenting factors from different perspectives such as management, user, processing, service pipeline, and data perspective. Moran et al. [77] assessed the impact of data quality by performing specific data preprocessings, and found that the significance of selecting a classifier decreases after applying an appropriate preprocessing step.

Within software engineering, data quality attributes have been extensively studied as mentioned in Section 2; however, our research is the first to empirically analyze the prevalence and impact of multiple data quality antipatterns in defect prediction. Moreover, to the best of our knowledge, no study has yet focused on the impact of antipatterns on model interpretation.

2. **Data quality issues in other domains.** The challenges in data quality for ML were identified as early as 1993 [78]. Data quality has been studied for different domains. For instance, Gupta et al.[79] analyzed data quality issues that led to sub-optimal ML models used in banking systems. Kerr et al.[80] presented a case study of data quality and its critical nature in the healthcare industry. For environment monitoring domain, Okafor et al. [81] developed an ML framework to monitor the quality of data for low-cost IoT Sensors. Our research builds upon these works by investigating data quality issues specifically in the software defect prediction domain. This focus allows us to identify unique challenges and opportunities in addressing data quality for software engineering applications, thereby contributing novel insights to the broader data quality literature.
3. **Data Quality Tools.** Several studies have proposed tools for monitoring the quality of data. For example, Grosso et al.[82] developed an ML-based tool for real-time monitoring particle detector data, and Ehrlinger et al.[83] proposed a DaQl (DATA Quality Library) as a generally-applicable tool to monitor the quality of data to increase the prediction accuracy of ML models. Similarly, Dai et al.[84] presented a framework built on deep learning and statistical models to identify data quality, and Shrivastava et al.[85] presented a toolkit for detecting, correcting, and explaining data quality for structured data. While these tools are valuable for general data quality monitoring, our research specifically examines the impact of data quality antipatterns in the software defect prediction domain. By focusing on this particular area, we contribute to the development of more targeted and effective data quality tools and strategies that cater to the specific challenges of software defect prediction.

*Aadi: [TODO: add this reference as suggested by bram: <https://dl.acm.org/doi/pdf/10.1145/1595696.1595716>]*

## 7 Implications

*Aadi: [still need to rewrite THIS again!] Aadi: [overall need to talk to Bram, since the entire results dont indicate much very authoritatively, we have too many experiments but no clear results.]* In this paper, we study the prevalence and impact of data quality antipatterns on the case study of Software Defect Prediction dataset. We present the key contributions of our study below:

- **Researchers and practitioners can leverage our taxonomy of data quality antipatterns as a checklist to qualify the prevalence and removal of antipatterns in their datasets.** We procured taxonomy of seven antipatterns (i.e., *Schema Violations*, *Data Misencoding*, *Inconsistent Representation*, *Data Distribution Antipatterns*, *Packaging Errors*, *Label Antipatterns*, and *Correlation & Redundancy*) along with 12 sub-types, ~~that~~ *which can* have potential impact on building machine learning models. Such a taxonomy can help data scientists in cleaning their datasets, by providing them with a checklist of antipatterns that may be important for their use case.
  - **Our schema for software defect prediction dataset helps future SDP researchers and practitioners clean schema violations in their SDP datasets.** In Section 3, we develop a schema for the SDP dataset. Such a schema not only helps software researchers but also encourages data scientists/engineers to check for and remove questionable or incorrect values in their datasets. *→ not much a big contribution?*
  - **SDP practitioners should not be overly concerned about the order of cleaning antipatterns while dealing with data cleaning for ML tasks.** From our **RQ2**, since the likelihood of a given order outperforming its inverse order is close to 50%, order does not seem to matter much in our results. This indicates that SDP researchers and practitioners can focus more on exploring other data preprocessing methods and their impact on model performance, without investing time and effort in figuring the optimal order of cleaning data quality antipatterns.
  - **SDP practitioners and researchers may wish to leverage our results of impact of antipatterns for prioritizing data cleaning efforts.** In **RQ3**, we observed that different antipatterns have different impacts on different performance metrics. Hence, practitioners can triage the antipattern cleaning based on the use case their SDP models.
- While removing class overlapped rows decreased the performance of our SDP models, it also overshadowed the impact of other antipatterns (as shown in Sec. 8). This knowledge can help practitioners by helping them focus on creating ML models robust to the presence of specific antipatterns, while prioritizing their efforts on problematic antipatterns.
- Finally, our results can help inform feature engineering and selection. SDP practitioners and researchers can make informed decisions about feature engineering and selection, especially when dealing with correlated and redundant features. This can lead to more efficient and accurate models.
- *Bram: [what about other software analytics researches?]*

## 8 Discussion

In this section, we provide a more detailed analysis of the results obtained in **RQ3**. Specifically, we did not observe any impact of mislabels on the performance of SDP models. Since this result contradicts prior research [32], we conduct further analysis to support our findings. Thus, in this subsection, we examine the inter-relationships between different antipatterns to explain our finding that Mislabeling has no effect on model performance.

**Approach.** In **RQ1**, we found that 94% of row-level antipattern overlaps are due to *Mislabel* and *Class Overlap* antipatterns. This indicates the need to examine the impact of class overlap on mislabel correction. Hence, we obtained AU-ROC results from models trained on five scenarios: *FiTrOv*, where mislabel correction is not performed; *FiTrMi*, where mislabel correction is performed but class overlapping rows are not removed; *FiTrOvMi*, where both class overlapping rows and mislabels are removed; *FiTrMiOv*, where both class overlapping rows and mislabels are removed, but the removal of class overlapping rows is based on incorrect labels; and *FiTr*, where neither class overlapping rows nor mislabels are corrected. Since Filter and Transformation based antipatterns do not have much significant impact from our **RQ3** findings, our *FiTr* and *FiTrMi* cases are comparable to Yatish et al.’s [32] experimental setup. To compare our findings to theirs, we only used the AU-ROC metric in this subsection.

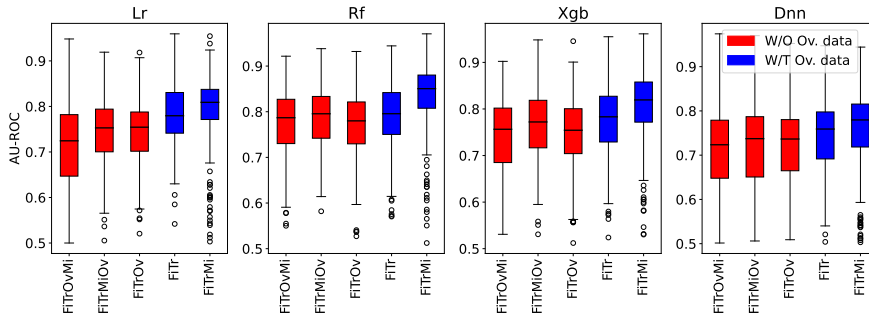

Fig. 13: Impact of Class Overlap removal on Mislabels. For ease of interpretation, red boxes show the removal of class overlapped rows, while the two blue boxes show replication of Yatish’s [32] experiments with and without Mislabels.

**Results: Removing class-overlapping rows reveals that the impact of mislabeling is overshadowed.** *Bram:* [is that good or bad?] *Aadi:* [Label quality is an important and active area of research. Potential implication is that once class overlap is removed, we may not have to worry too much on label quality if class overlap is done. Altho, I can’t say that authoritatively unless I have

*show the same phenomenon via few more datasets.]* Figure 13 shows orders with class-overlapping rows removed in red and orders with class-overlapping rows present in blue. The blue boxes indicate that mislabeling significantly affects the model’s AU-ROC, as previously identified by Yatish et al. [32]. The order *FiTr* exhibits a lower AU-ROC than the order *FiTrMi*, where mislabel correction is performed. This observation is supported by statistically significant comparisons (Wilcoxon Rank-Sum test,  $p - value \leq 0.05$ ) with small to medium effect sizes.

However, when class-overlapping rows are removed (i.e., red boxes in Figure 13), the orders *FiTrOvMi* and *FiTrMiOv* do not exhibit a very distinct AU-ROC compared to *FiMiOv*, which demonstrates the diminished impact of mislabeling. This is further evidenced by statistically insignificant differences (Wilcoxon Rank-Sum test,  $p - value \leq 0.05$ ) between *FiTrOv* and *FiTrOvMi* with a medium to large effect sizes for three out of four classifiers, accompanied by a small effect size (Cliff’s  $\delta = -0.19$ ) for the remaining classifier, Logistic Regression.

→ what does all this mean?

## 9 Conclusion

In this paper, we present a comprehensive investigation of data quality antipatterns. Our research provides a better understanding of the prevalence, impact, and influence of these antipatterns on the performance and interpretation of machine learning models used for software defect prediction.

We demonstrate that data quality antipatterns are prevalent in software defect prediction datasets, while presence of only two antipatterns, *class overlap* and *tailed features* can affect the model’s performance. Moreover, practitioners shouldn’t be too concerned about the order of cleaning multiple antipatterns. Overall, our findings highlight the importance of focusing efforts for data quality issues management in SDP applications.

Furthermore, we explore the impact of antipatterns on model interpretation, revealing that the consistency of interpretation can be moderately affected by the presence of these antipatterns. This finding underscores the importance of considering data quality when interpreting machine learning models in the software defect prediction domain, moderately impact the reliability of insights for decision-making.

Our research contributes to the existing body of literature on data quality in software engineering and software defect prediction by providing novel insights into the role of data quality antipatterns in model performance and interpretation. Moreover, our work helps pave the way for the development of targeted strategies and tools for addressing data quality issues in the software defect prediction domain, thereby enhancing the reliability and effectiveness of machine learning models in this context.

In future work, we plan to extend our analysis to other software engineering tasks and investigate additional data quality antipatterns to further understand their impact on machine learning applications. Additionally, we aim

to develop specific techniques and best practices for mitigating the negative effects of data and label quality, ultimately improving the overall performance and interpretability of machine learning models in this domain.

## References

1. P. Domingos, “A few useful things to know about machine learning,” *Communications of the ACM*, vol. 55, no. 10, pp. 78–87, 2012.
2. M. Shepperd, Q. Song, Z. Sun, and C. Mair, “Data quality: Some comments on the nasa software defect datasets,” *IEEE Transactions on Software Engineering*, vol. 39, no. 9, pp. 1208–1215, 2013.
3. A. Sharma and P. K. Mishra, “Performance analysis of machine learning based optimized feature selection approaches for breast cancer diagnosis,” *International Journal of Information Technology*, vol. 14, no. 4, pp. 1949–1960, 2022.
4. E. Breck, N. Polyzotis, S. Roy, S. Whang, and M. Zinkevich, “Data validation for machine learning,” in *MLSys*, 2019.
5. I. Žliobaitė, M. Pechenizkiy, and J. Gama, “An overview of concept drift applications,” *Big data analysis: new algorithms for a new society*, pp. 91–114, 2016.
6. L. Chen, B. Fang, Z. Shang, and Y. Tang, “Tackling class overlap and imbalance problems in software defect prediction,” *Software Quality Journal*, vol. 26, no. 1, pp. 97–125, 2018.
7. M. Denil and T. Trappenberg, “Overlap versus imbalance,” in *Canadian conference on artificial intelligence*. Springer, 2010, pp. 220–231.
8. P. Vuttipittayamongkol, E. Elyan, and A. Petrovski, “On the class overlap problem in imbalanced data classification,” *Knowledge-based systems*, vol. 212, p. 106631, 2021.
9. L. Gong, S. Jiang, R. Wang, and L. Jiang, “Empirical evaluation of the impact of class overlap on software defect prediction,” in *2019 34th IEEE/ACM International Conference on Automated Software Engineering (ASE)*. IEEE, 2019, pp. 698–709.
10. J. M. Johnson and T. M. Khoshgoftaar, “Survey on deep learning with class imbalance,” *Journal of Big Data*, vol. 6, no. 1, pp. 1–54, 2019.
11. Y. Yang and Z. Xu, “Rethinking the value of labels for improving class-imbalanced learning,” *Advances in neural information processing systems*, vol. 33, pp. 19 290–19 301, 2020.
12. H. Ali, M. N. M. Salleh, R. Saedudin, K. Hussain, and M. F. Mushtaq, “Imbalance class problems in data mining: a review,” *Indonesian Journal of Electrical Engineering and Computer Science*, vol. 14, no. 3, pp. 1560–1571, 2019.
13. J. I. Daoud, “Multicollinearity and regression analysis,” in *Journal of Physics: Conference Series*, vol. 949, no. 1. IOP Publishing, 2017, p. 012009.
14. S. McIntosh, Y. Kamei, B. Adams, and A. E. Hassan, “An empirical study of the impact of modern code review practices on software quality,” *Empirical Software Engineering*, vol. 21, no. 5, pp. 2146–2189, 2016.
15. R. Gitzel, “Data quality in time series data: An experience report,” in *CBI (Industrial Track)*, 2016, pp. 41–49.
16. S. Ackerman, E. Farchi, O. Raz, M. Zalmanovici, and P. Dube, “Detection of data drift and outliers affecting machine learning model performance over time,” *arXiv preprint arXiv:2012.09258*, 2020.
17. N. Hynes, D. Sculley, and M. Terry, “The data linter: Lightweight, automated sanity checking for ml data sets,” in *NIPS MLSys Workshop*, vol. 1, 2017.
18. D. Rajapaksha, C. Tantithamthavorn, J. Jiarapakdee, C. Bergmeir, J. Grundy, and W. Buntine, “Sqaplanner: Generating data-informed software quality improvement plans,” *IEEE Transactions on Software Engineering*, vol. 48, no. 8, pp. 2814–2835, 2021.
19. J. Jiarapakdee, C. K. Tantithamthavorn, and J. Grundy, “Practitioners’ perceptions of the goals and visual explanations of defect prediction models,” in *2021 IEEE/ACM 18th International Conference on Mining Software Repositories (MSR)*. IEEE, 2021, pp. 432–443.

20. H. Tong, B. Liu, and S. Wang, "Kernel spectral embedding transfer ensemble for heterogeneous defect prediction," *IEEE Transactions on Software Engineering*, vol. 47, no. 9, pp. 1886–1906, 2019.
21. L. Gong, G. K. Rajbahadur, A. E. Hassan, and S. Jiang, "Revisiting the impact of dependency network metrics on software defect prediction," *IEEE Transactions on Software Engineering*, vol. 48, no. 12, pp. 5030–5049, 2021.
22. R. Moussa and F. Sarro, "On the use of evaluation measures for defect prediction studies," in *Proceedings of the 31st ACM SIGSOFT International Symposium on Software Testing and Analysis*, 2022, pp. 101–113.
23. J. Jiarpakdee, C. K. Tantithamthavorn, H. K. Dam, and J. Grundy, "An empirical study of model-agnostic techniques for defect prediction models," *IEEE Transactions on Software Engineering*, vol. 48, no. 1, pp. 166–185, 2020.
24. S. Wattanakriengkrai, P. Thongtanunam, C. Tantithamthavorn, H. Hata, and K. Matsumoto, "Predicting defective lines using a model-agnostic technique," *IEEE Transactions on Software Engineering*, vol. 48, no. 5, pp. 1480–1496, 2020.
25. M. Fu and C. Tantithamthavorn, "Linevul: A transformer-based line-level vulnerability prediction," in *Proceedings of the 19th International Conference on Mining Software Repositories*, 2022, pp. 608–620.
26. G. I. Webb, R. Hyde, H. Cao, H. L. Nguyen, and F. Petitjean, "Characterizing concept drift," *Data Mining and Knowledge Discovery*, vol. 30, no. 4, pp. 964–994, 2016.
27. S. Amershi, A. Begel, C. Bird, R. DeLine, H. Gall, E. Kamar, N. Nagappan, B. Nushi, and T. Zimmermann, "Software engineering for machine learning: A case study," in *2019 IEEE/ACM 41st International Conference on Software Engineering: Software Engineering in Practice (ICSE-SEIP)*. IEEE, 2019, pp. 291–300.
28. T. Emmanuel, T. Maupong, D. Mpoeleng, T. Semong, B. Mphago, and O. Tabona, "A survey on missing data in machine learning," *Journal of Big Data*, vol. 8, no. 1, pp. 1–37, 2021.
29. I. F. Ilyas and X. Chu, *Data cleaning*. Morgan & Claypool, 2019.
30. L. Eadicicco, "He Helped Create the 'Google Brain.' Here's What He Thinks About AI Now," <https://time.com/4631730/andrew-ng-artificial-intelligence-2017/>, 2017, [Online; Retrieved 1-February-2023].
31. D. A. Da Costa, S. McIntosh, W. Shang, U. Kulesza, R. Coelho, and A. E. Hassan, "A framework for evaluating the results of the szz approach for identifying bug-introducing changes," *IEEE Transactions on Software Engineering*, vol. 43, no. 7, pp. 641–657, 2016.
32. S. Yatish, J. Jiarpakdee, P. Thongtanunam, and C. Tantithamthavorn, "Mining software defects: Should we consider affected releases?" in *2019 IEEE/ACM 41st International Conference on Software Engineering (ICSE)*. IEEE, 2019, pp. 654–665.
33. X. Guo, Y. Yin, C. Dong, G. Yang, and G. Zhou, "On the class imbalance problem," in *2008 Fourth international conference on natural computation*, vol. 4. IEEE, 2008, pp. 192–201.
34. J. Jiarpakdee, C. Tantithamthavorn, and A. Hassan, "The impact of correlated metrics on the interpretation of defect prediction models," *IEEE Trans. Software Eng. early access*, vol. 10, 2019.
35. G. K. Rajbahadur, S. Wang, G. A. Oliva, Y. Kamei, and A. E. Hassan, "The impact of feature importance methods on the interpretation of defect classifiers," *IEEE Transactions on Software Engineering*, vol. 48, no. 7, pp. 2245–2261, 2021.
36. N. S. Harzevili and S. H. Alizadeh, "Analysis and modeling conditional mutual dependency of metrics in software defect prediction using latent variables," *Neurocomputing*, vol. 460, pp. 309–330, 2021.
37. E. Debie and K. Shafi, "Implications of the curse of dimensionality for supervised learning classifier systems: theoretical and empirical analyses," *Pattern Analysis and Applications*, vol. 22, pp. 519–536, 2019.
38. W. K. Vong, A. T. Hendrickson, D. J. Navarro, and A. Perfors, "Do additional features help or hurt category learning? the curse of dimensionality in human learners," *Cognitive science*, vol. 43, no. 3, p. e12724, 2019.
39. N. Pudjihartono, T. Fadason, A. W. Kempa-Liehr, and J. M. O'Sullivan, "A review of feature selection methods for machine learning-based disease risk prediction," *Frontiers in Bioinformatics*, vol. 2, p. 927312, 2022.

40. T. Hastie, R. Tibshirani, J. H. Friedman, and J. H. Friedman, *The elements of statistical learning: data mining, inference, and prediction*. Springer, 2009, vol. 2.
41. A. L'heureux, K. Grolinger, H. F. Elyamany, and M. A. Capretz, "Machine learning with big data: Challenges and approaches," *Ieee Access*, vol. 5, pp. 7776–7797, 2017.
42. Y. Kamei, E. Shihab, B. Adams, A. E. Hassan, A. Mockus, A. Sinha, and N. Ubayashi, "A large-scale empirical study of just-in-time quality assurance," *IEEE Transactions on Software Engineering*, vol. 39, no. 6, pp. 757–773, 2012.
43. M. D'Ambros, M. Lanza, and R. Robbes, "Evaluating defect prediction approaches: a benchmark and an extensive comparison," *Empirical Software Engineering*, vol. 17, no. 4, pp. 531–577, 2012.
44. W. Tang and T. M. Khoshgoftaar, "Noise identification with the k-means algorithm," in *16th IEEE International Conference on Tools with Artificial Intelligence*. IEEE, 2004, pp. 373–378.
45. J. Jiarpakdee and C. Tantithamthavorn, "Rnalytica: An r package of jira defect datasets and tool suites for explainable software analytics," <https://github.com/awsm-research/Rnalytica>.
46. J. Jiarpakdee, C. Tantithamthavorn, and C. Treude, "Autospearman: Automatically mitigating correlated software metrics for interpreting defect models," in *2018 IEEE International Conference on Software Maintenance and Evolution (ICSME)*. IEEE Computer Society, 2018, pp. 92–103.
47. J. Tan, D. Feitosa, and P. Avgeriou, "Does it matter who pays back technical debt? an empirical study of self-fixed td," *Information and Software Technology*, vol. 143, p. 106738, 2022.
48. S. Hassan, C. Tantithamthavorn, C.-P. Bezemer, and A. E. Hassan, "Studying the dialogue between users and developers of free apps in the google play store," *Empirical Software Engineering*, vol. 23, no. 3, pp. 1275–1312, 2018.
49. C. Tantithamthavorn, S. McIntosh, A. E. Hassan, and K. Matsumoto, "Automated parameter optimization of classification techniques for defect prediction models," in *Proceedings of the 38th international conference on software engineering*, 2016, pp. 321–332.
50. R. M. Yasir, M. Asad, and D. A. Kabir, "Defect prediction using stylistic metrics," *arXiv preprint arXiv:2206.10959*, 2022.
51. P. Khakhar and R. K. Dubey, "The integrity of machine learning algorithms against software defect prediction," in *Artificial Intelligence and Machine Learning for EDGE Computing*. Elsevier, 2022, pp. 65–74.
52. J. Bergstra and Y. Bengio, "Random search for hyper-parameter optimization," *Journal of machine learning research*, vol. 13, no. 2, 2012.
53. A. Agrawal, X. Yang, R. Agrawal, R. Yedida, X. Shen, and T. Menzies, "Simpler hyperparameter optimization for software analytics: why, how, when," *IEEE Transactions on Software Engineering*, 2021.
54. A. Alazba and H. Aljamaan, "Software defect prediction using stacking generalization of optimized tree-based ensembles," *Applied Sciences*, vol. 12, no. 9, p. 4577, 2022.
55. R. B. Bahaweres, F. Agustian, I. Hermadi, A. I. Suroso, and Y. Arkeman, "Software defect prediction using neural network based smote," in *2020 7th International Conference on Electrical Engineering, Computer Sciences and Informatics (EECSI)*. IEEE, 2020, pp. 71–76.
56. J. Davis and M. Goadrich, "The relationship between precision-recall and roc curves," in *Proceedings of the 23rd international conference on Machine learning*, 2006, pp. 233–240.
57. D. Chicco and G. Jurman, "The advantages of the matthews correlation coefficient (mcc) over f1 score and accuracy in binary classification evaluation," *BMC genomics*, vol. 21, pp. 1–13, 2020.
58. C. Tantithamthavorn and A. E. Hassan, "An experience report on defect modelling in practice: Pitfalls and challenges," in *Proceedings of the 40th international conference on software engineering: Software engineering in practice*, 2018, pp. 286–295.
59. C. K. Tantithamthavorn and J. Jiarpakdee, "Explainable ai for software engineering," in *2021 36th IEEE/ACM International Conference on Automated Software Engineering (ASE)*. IEEE, 2021, pp. 1–2.

60. X. Wu, W. Zheng, X. Xia, and D. Lo, "Data quality matters: A case study on data label correctness for security bug report prediction," *IEEE Transactions on Software Engineering*, vol. 48, no. 7, pp. 2541–2556, 2021.
61. Z. Qi, H. Wang, J. Li, and H. Gao, "Impacts of dirty data: and experimental evaluation," *arXiv preprint arXiv:1803.06071*, 2018.
62. B. Frénay and M. Verleysen, "Classification in the presence of label noise: a survey," *IEEE transactions on neural networks and learning systems*, vol. 25, no. 5, pp. 845–869, 2013.
63. J. Bootkrajang and A. Kabán, "Label-noise robust logistic regression and its applications," in *Machine Learning and Knowledge Discovery in Databases: European Conference, ECML PKDD 2012, Bristol, UK, September 24–28, 2012. Proceedings, Part I* 23. Springer, 2012, pp. 143–158.
64. A. Halevy, P. Norvig, and F. Pereira, "The unreasonable effectiveness of data," *IEEE intelligent systems*, vol. 24, no. 2, pp. 8–12, 2009.
65. A. Bhatia, E. E. Eghan, M. Grichi, W. G. Cavanagh, Z. Ming, B. Adams et al., "Towards a change taxonomy for machine learning systems," *arXiv preprint arXiv:2203.11365*, 2022.
66. C. Tantithamthavorn, S. McIntosh, A. E. Hassan, and K. Matsumoto, "An empirical comparison of model validation techniques for defect prediction models," *IEEE Transactions on Software Engineering*, vol. 43, no. 1, pp. 1–18, 2016.
67. N. Cliff, *Ordinal methods for behavioral data analysis*. Psychology Press, 2014.
68. Y. Lyu, H. Li, M. Sayagh, Z. M. Jiang, and A. E. Hassan, "An empirical study of the impact of data splitting decisions on the performance of aiops solutions," *ACM Transactions on Software Engineering and Methodology (TOSEM)*, vol. 30, no. 4, pp. 1–38, 2021.
69. Y. Lyu, G. K. Rajbahadur, D. Lin, B. Chen, and Z. M. Jiang, "Towards a consistent interpretation of aiops models," *ACM Transactions on Software Engineering and Methodology (TOSEM)*, vol. 31, no. 1, pp. 1–38, 2021.
70. L. Breiman, "Random forests," *Machine learning*, vol. 45, pp. 5–32, 2001.
71. M. T. Ribeiro, S. Singh, and C. Guestrin, "why should i trust you?" explaining the predictions of any classifier," in *Proceedings of the 22nd ACM SIGKDD international conference on knowledge discovery and data mining*, 2016, pp. 1135–1144.
72. T. Zimmermann, N. Nagappan, H. Gall, E. Giger, and B. Murphy, "Cross-project defect prediction: a large scale experiment on data vs. domain vs. process," in *Proceedings of the 7th joint meeting of the European software engineering conference and the ACM SIGSOFT symposium on The foundations of software engineering*, 2009, pp. 91–100.
73. A. Jain, H. Patel, L. Nagalapatti, N. Gupta, S. Mehta, S. Guttula, S. Mujumdar, S. Afzal, R. Sharma Mittal, and V. Munigala, "Overview and importance of data quality for machine learning tasks," in *Proceedings of the 26th ACM SIGKDD International Conference on Knowledge Discovery & Data Mining*, 2020, pp. 3561–3562.
74. N. Gupta, S. Mujumdar, H. Patel, S. Masuda, N. Panwar, S. Bandyopadhyay, S. Mehta, S. Guttula, S. Afzal, R. Sharma Mittal et al., "Data quality for machine learning tasks," in *Proceedings of the 27th ACM SIGKDD Conference on Knowledge Discovery & Data Mining*, 2021, pp. 4040–4041.
75. C. Renggli, L. Rımanic, N. M. Gürel, B. Karlaš, W. Wu, and C. Zhang, "A data quality-driven view of mlops," *arXiv preprint arXiv:2102.07750*, 2021.
76. M. Abdallah, "Big data quality challenges," in *2019 International Conference on Big Data and Computational Intelligence (ICBDICI)*. IEEE, 2019, pp. 1–3.
77. L. Morán-Fernández, V. Bólon-Canedo, and A. Alonso-Betanzos, "How important is data quality? best classifiers vs best features," *Neurocomputing*, vol. 470, pp. 365–375, 2022.
78. C. Cortes, L. D. Jackel, and W.-P. Chiang, "Limits on learning machine accuracy imposed by data quality," *Advances in Neural Information Processing Systems*, vol. 7, 1994.
79. A. Gupta, D. N. Dwivedi, J. Shah, and A. Jain, "Data quality issues leading to sub optimal machine learning for money laundering models," *Journal of Money Laundering Control*, vol. 25, no. 3, pp. 551–555, 2022.
80. K. Kerr, T. Norris, and R. Stockdale, "Data quality information and decision making: a healthcare case study," *ACIS 2007 Proceedings*, p. 98, 2007.



81. N. U. Okafor, Y. Alghorani, and D. T. Delaney, "Improving data quality of low-cost iot sensors in environmental monitoring networks using data fusion and machine learning approach," *ICT Express*, vol. 6, no. 3, pp. 220–228, 2020.
82. G. Grosso, N. Lai, M. Letizia, J. Pazzini, M. Rando, A. Wulzer, and M. Zanetti, "A fast and flexible machine learning approach to data quality monitoring," *arXiv preprint arXiv:2301.08917*, 2023.
83. L. Ehrlinger, V. Haunschmid, D. Palazzini, and C. Lettner, "A daql to monitor data quality in machine learning applications," in *Database and Expert Systems Applications: 30th International Conference, DEXA 2019, Linz, Austria, August 26–29, 2019, Proceedings, Part I 30*. Springer, 2019, pp. 227–237.
84. W. Dai, K. Yoshigoe, and W. Parsley, "Improving data quality through deep learning and statistical models," in *Information Technology-New Generations: 14th International Conference on Information Technology*. Springer, 2018, pp. 515–522.
85. S. Shrivastava, D. Patel, N. Zhou, A. Iyengar, and A. Bhamidipaty, "Dqlearn: a toolkit for structured data quality learning," in *2020 IEEE International Conference on Big Data (Big Data)*. IEEE, 2020, pp. 1644–1653.
